# Supplementary material for: Anomaly Detection by Effectively Leveraging Synthetic Images
Source: arXiv:2512.23227 source file (2025-12-29)
Supplement: Supplementary file 1 [file supmat_figure.pdf]

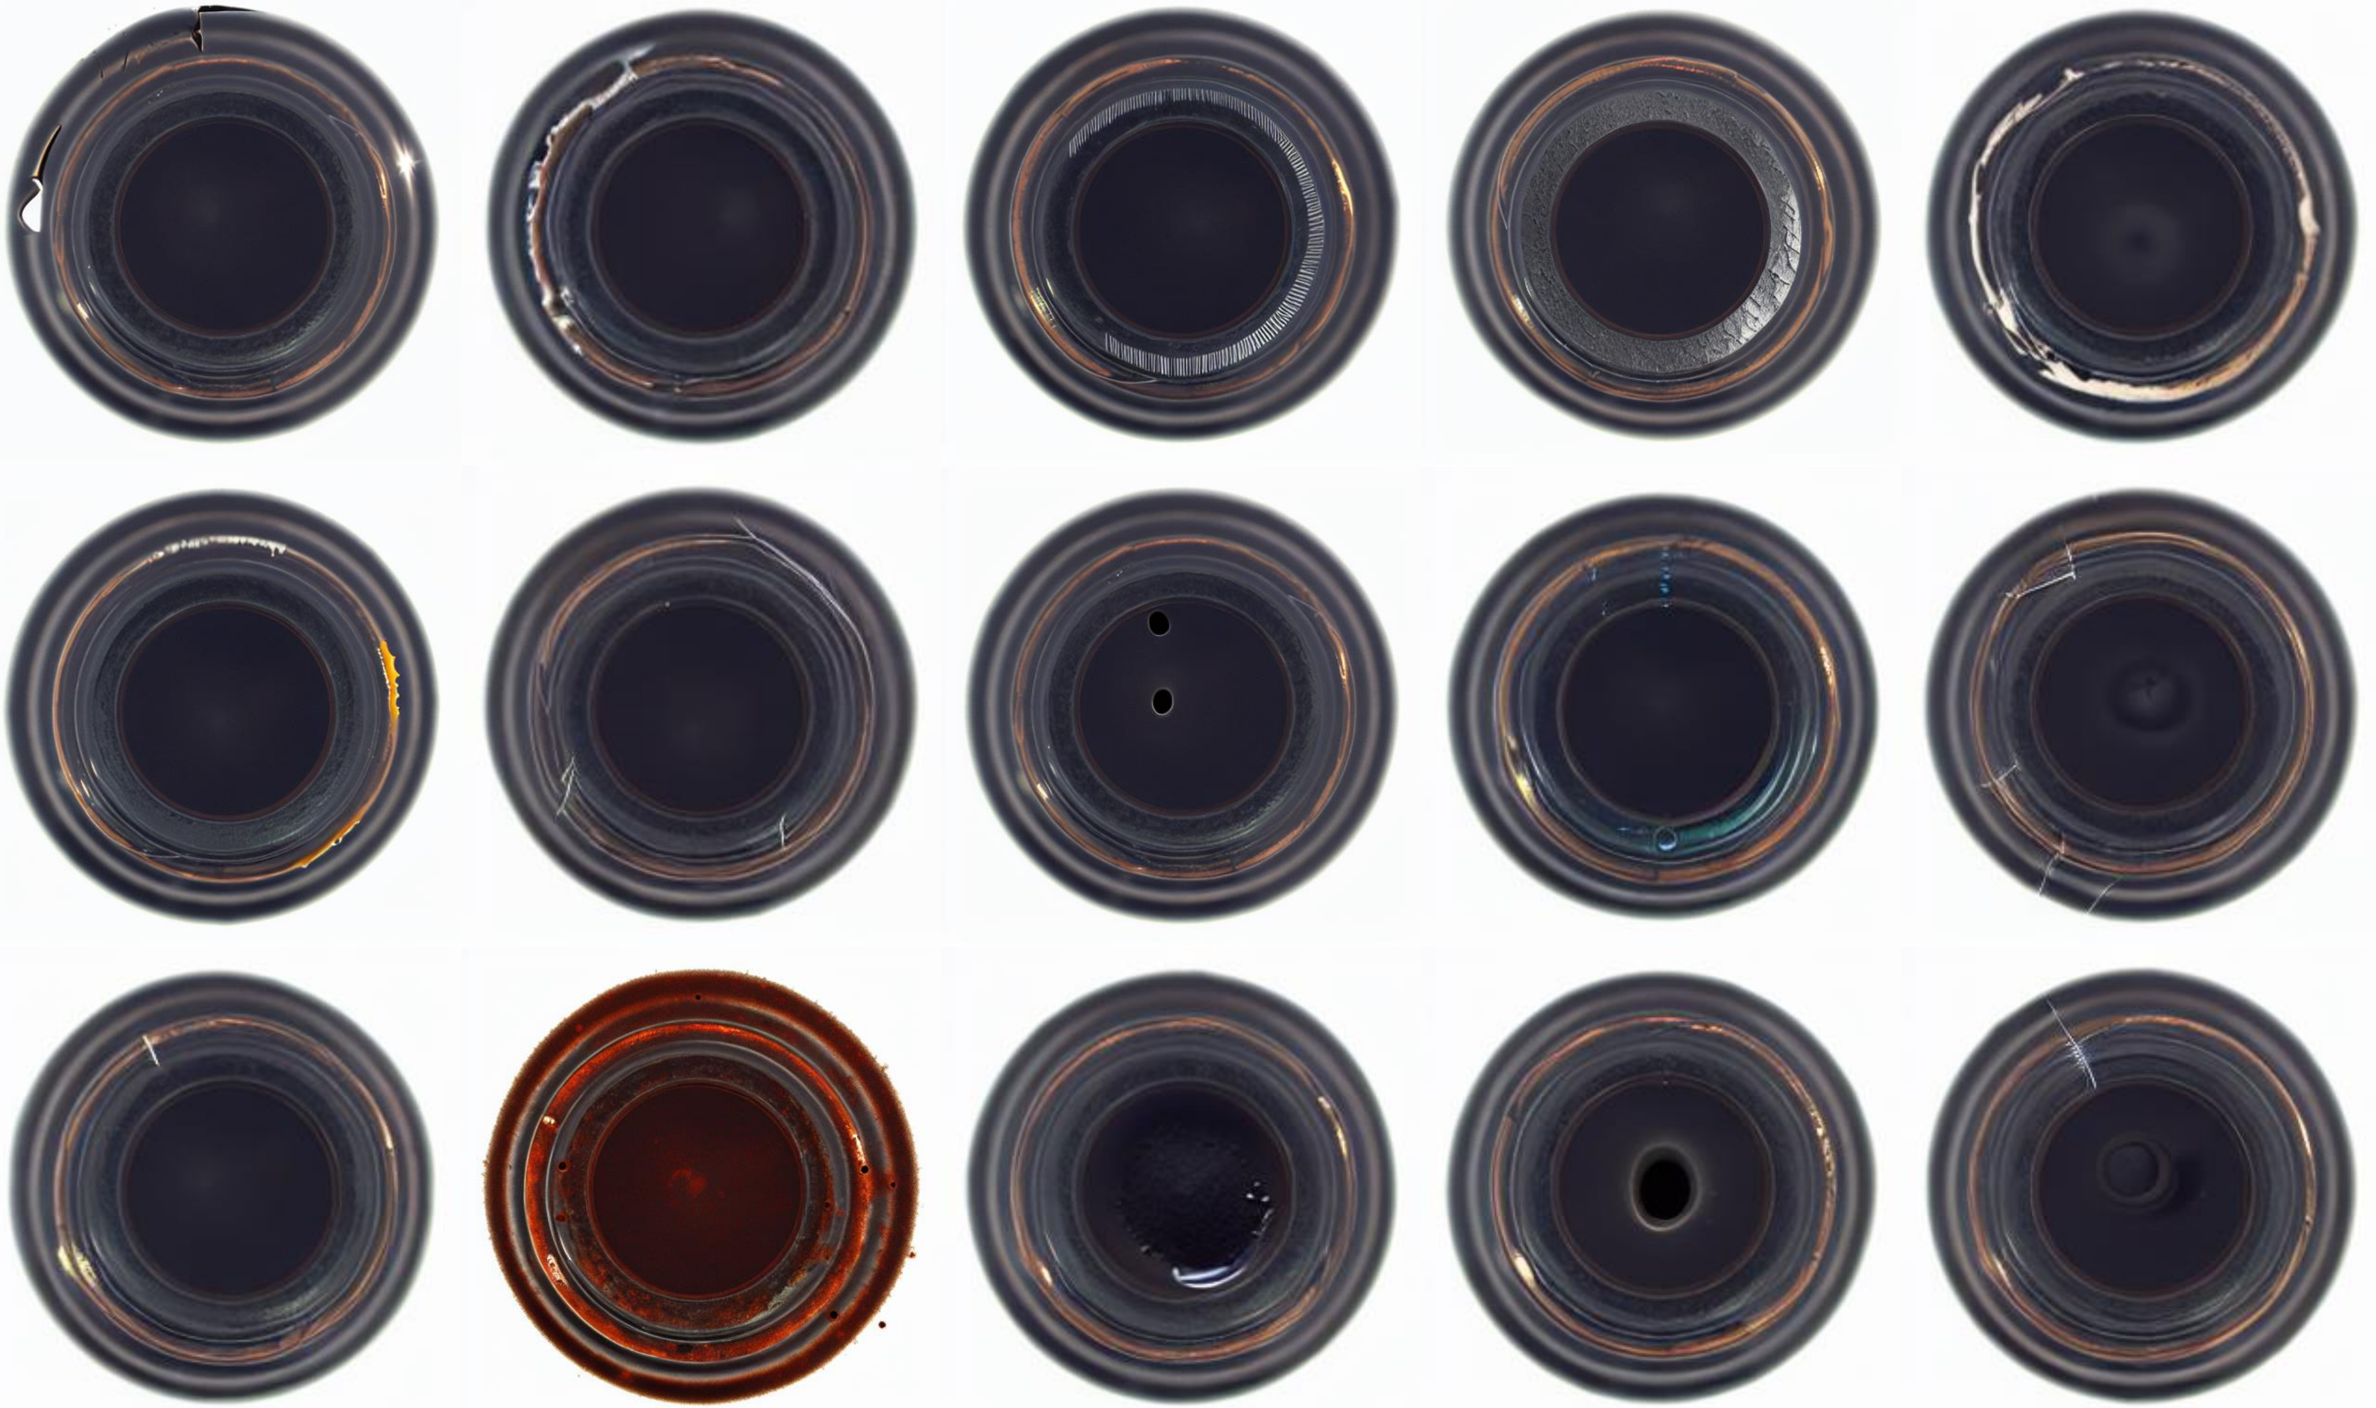

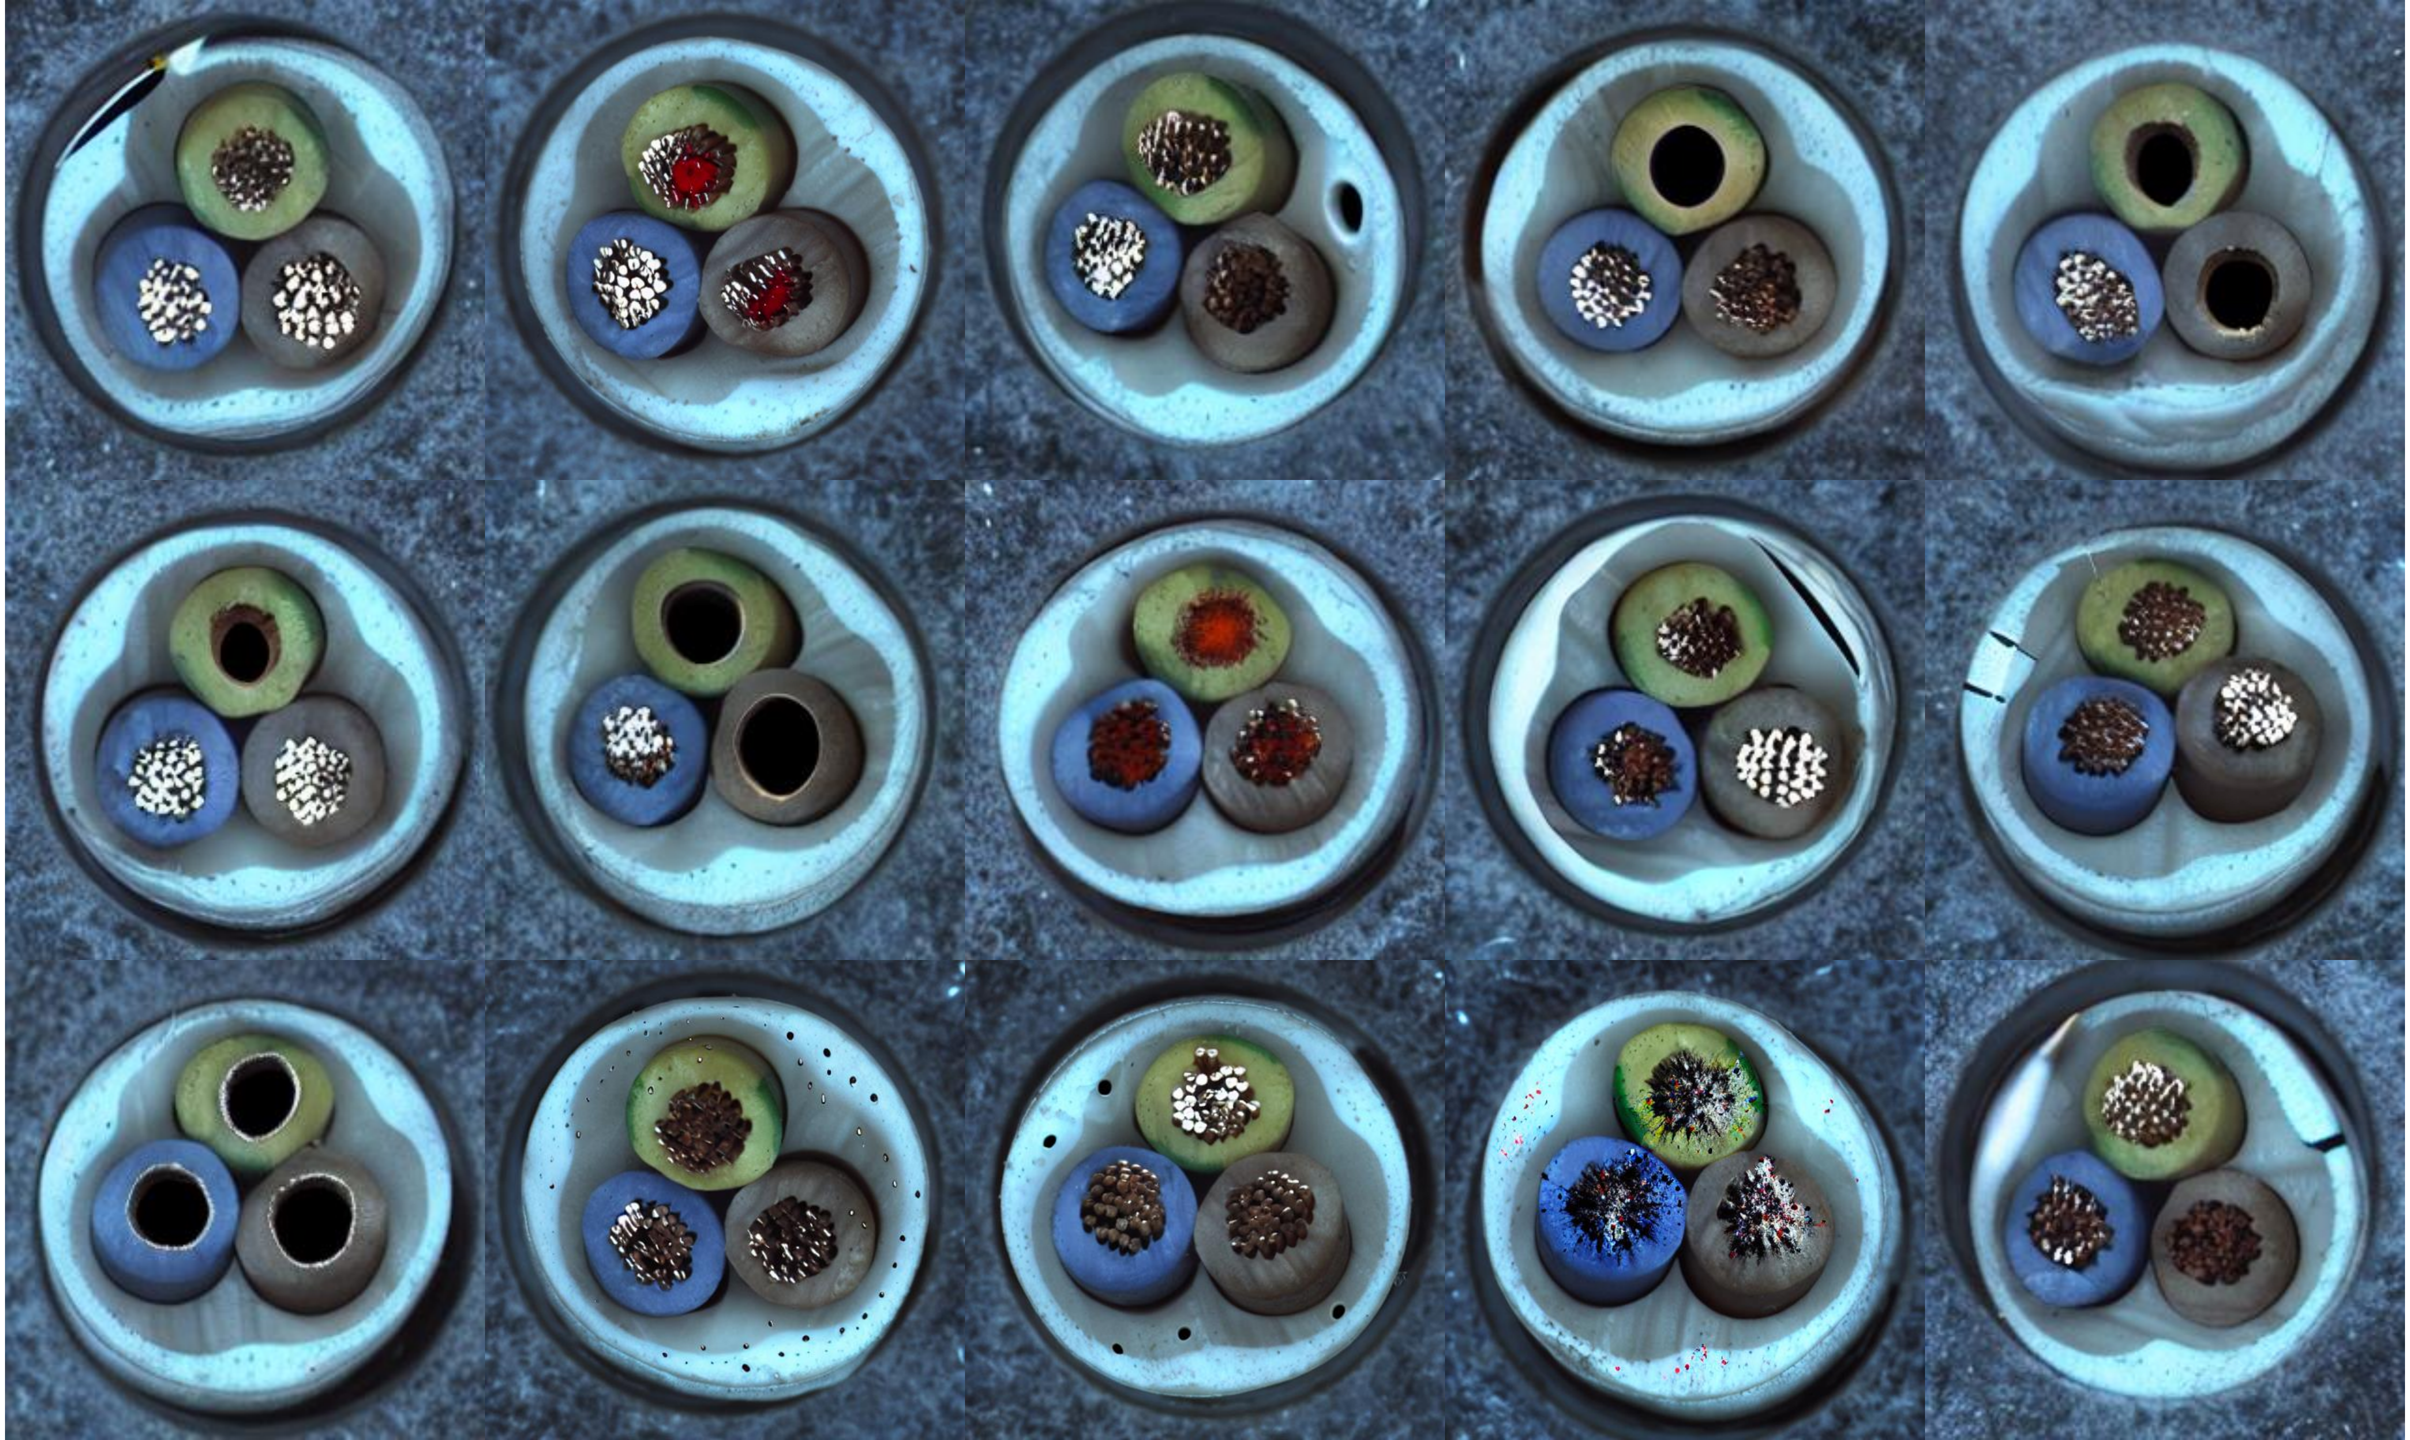

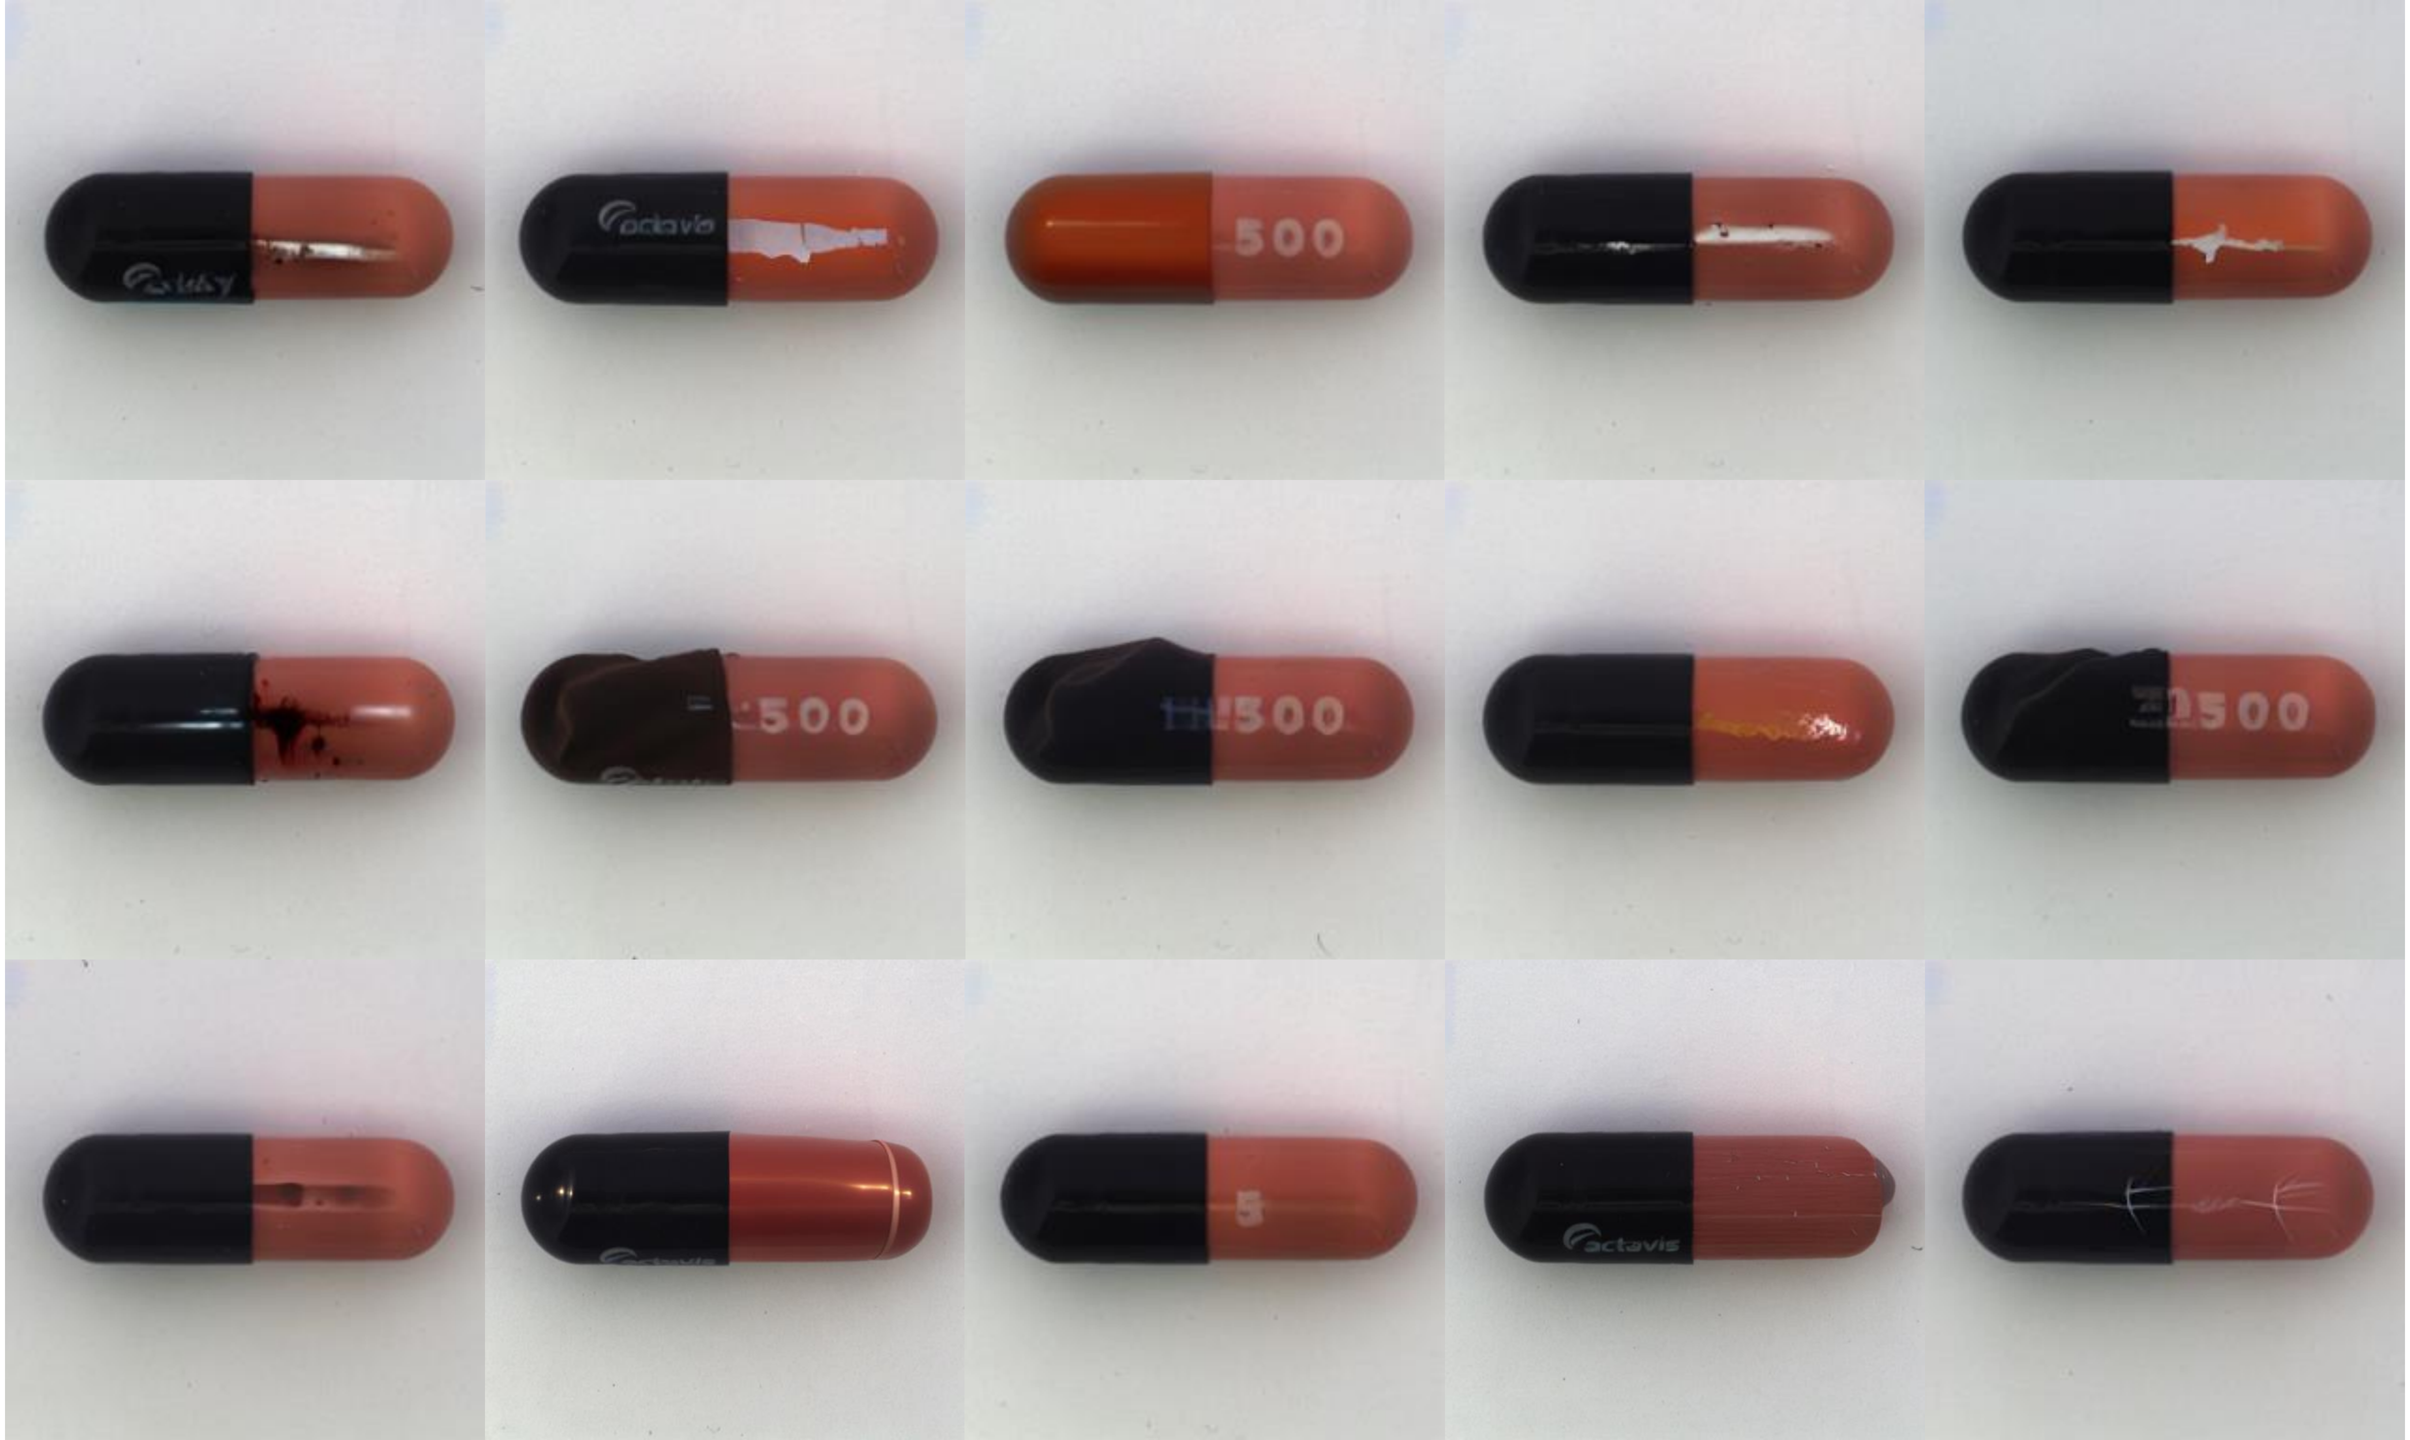
actavis
500
500
500
500
5
actavis

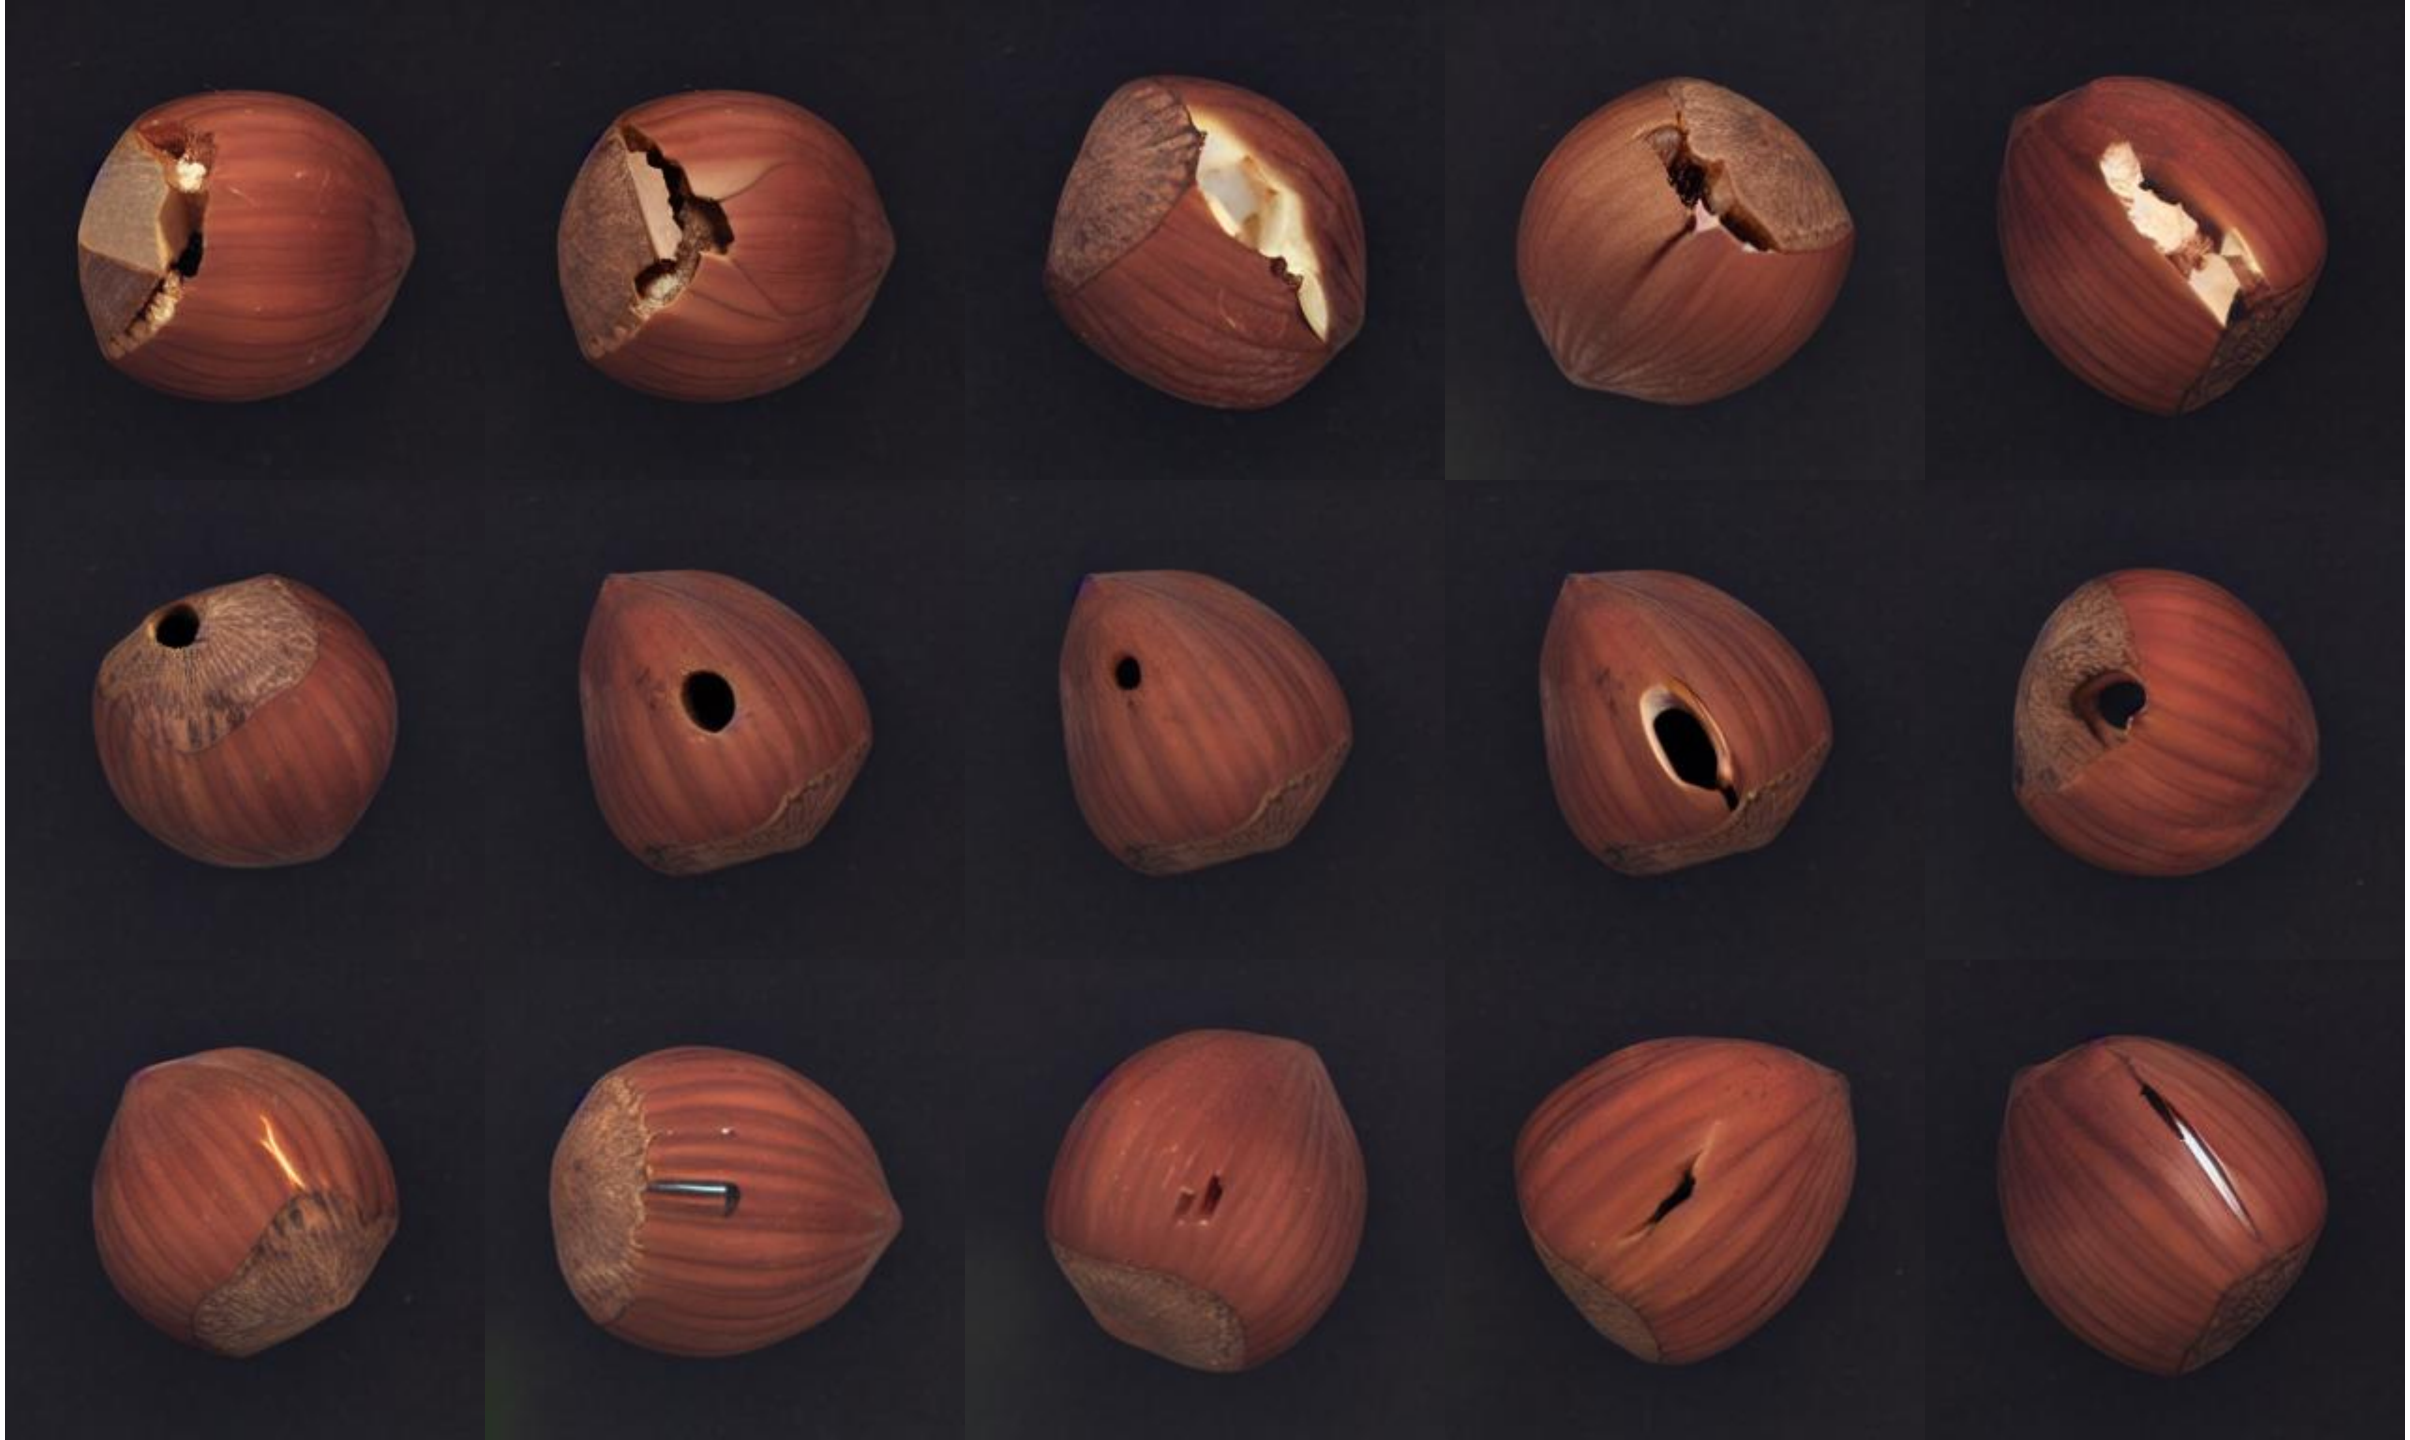

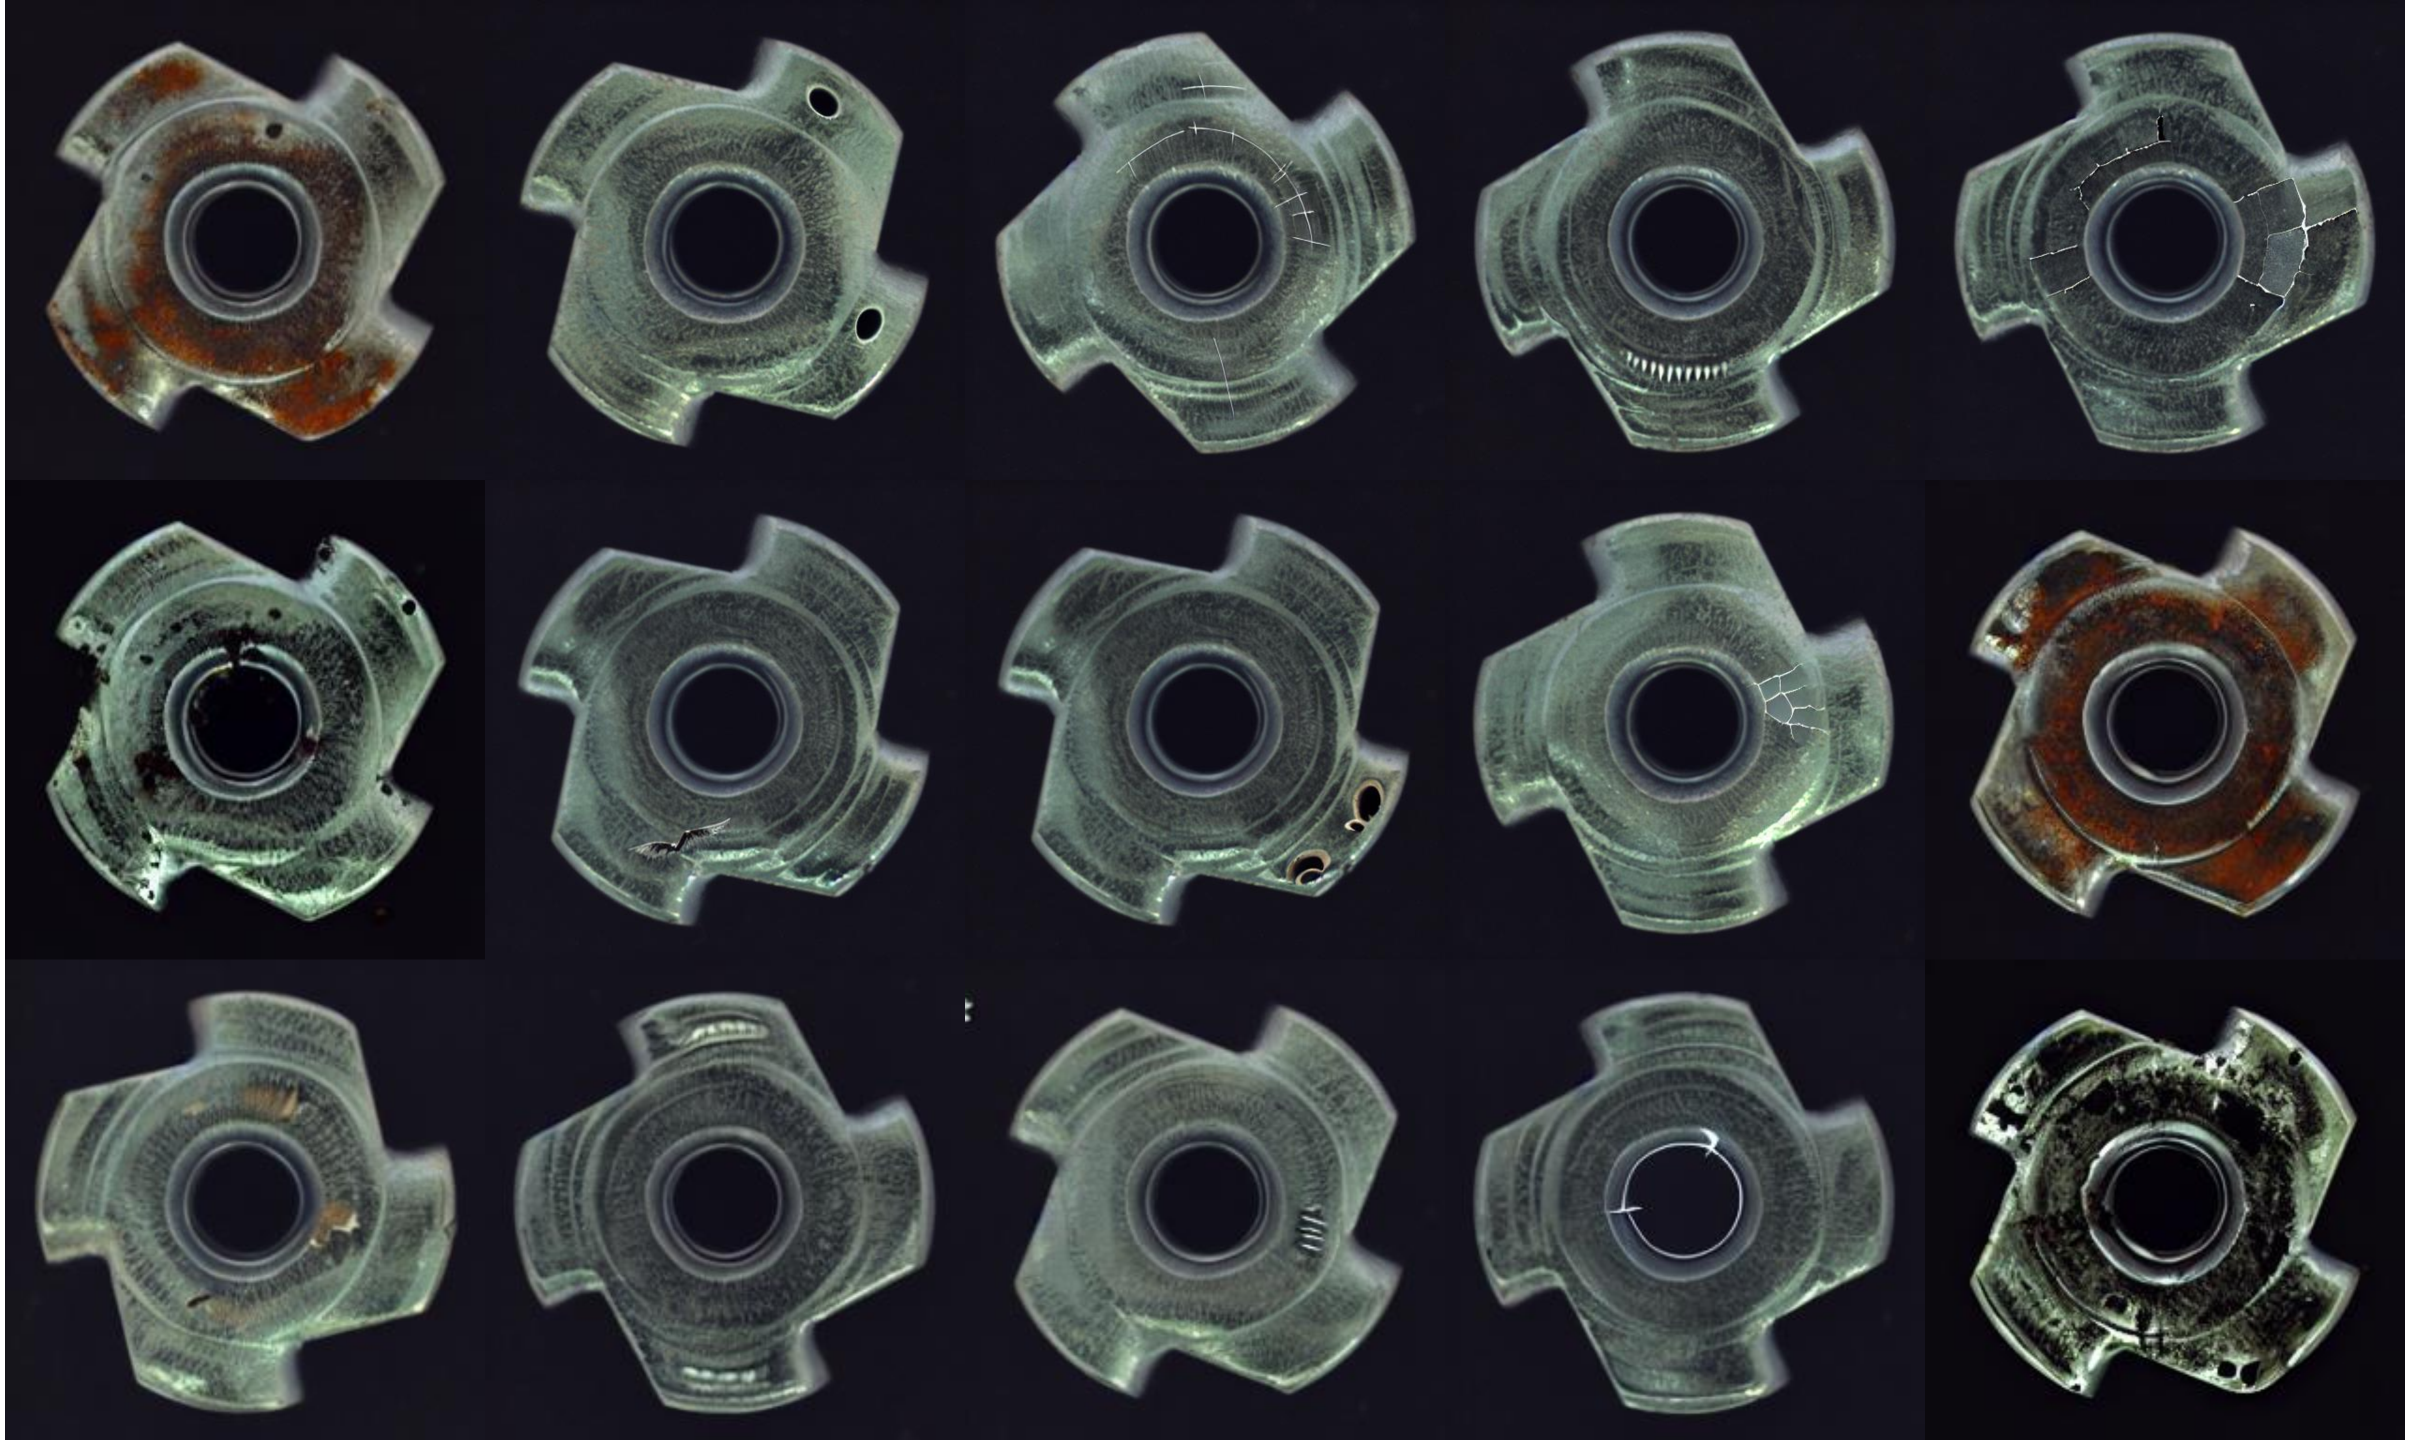

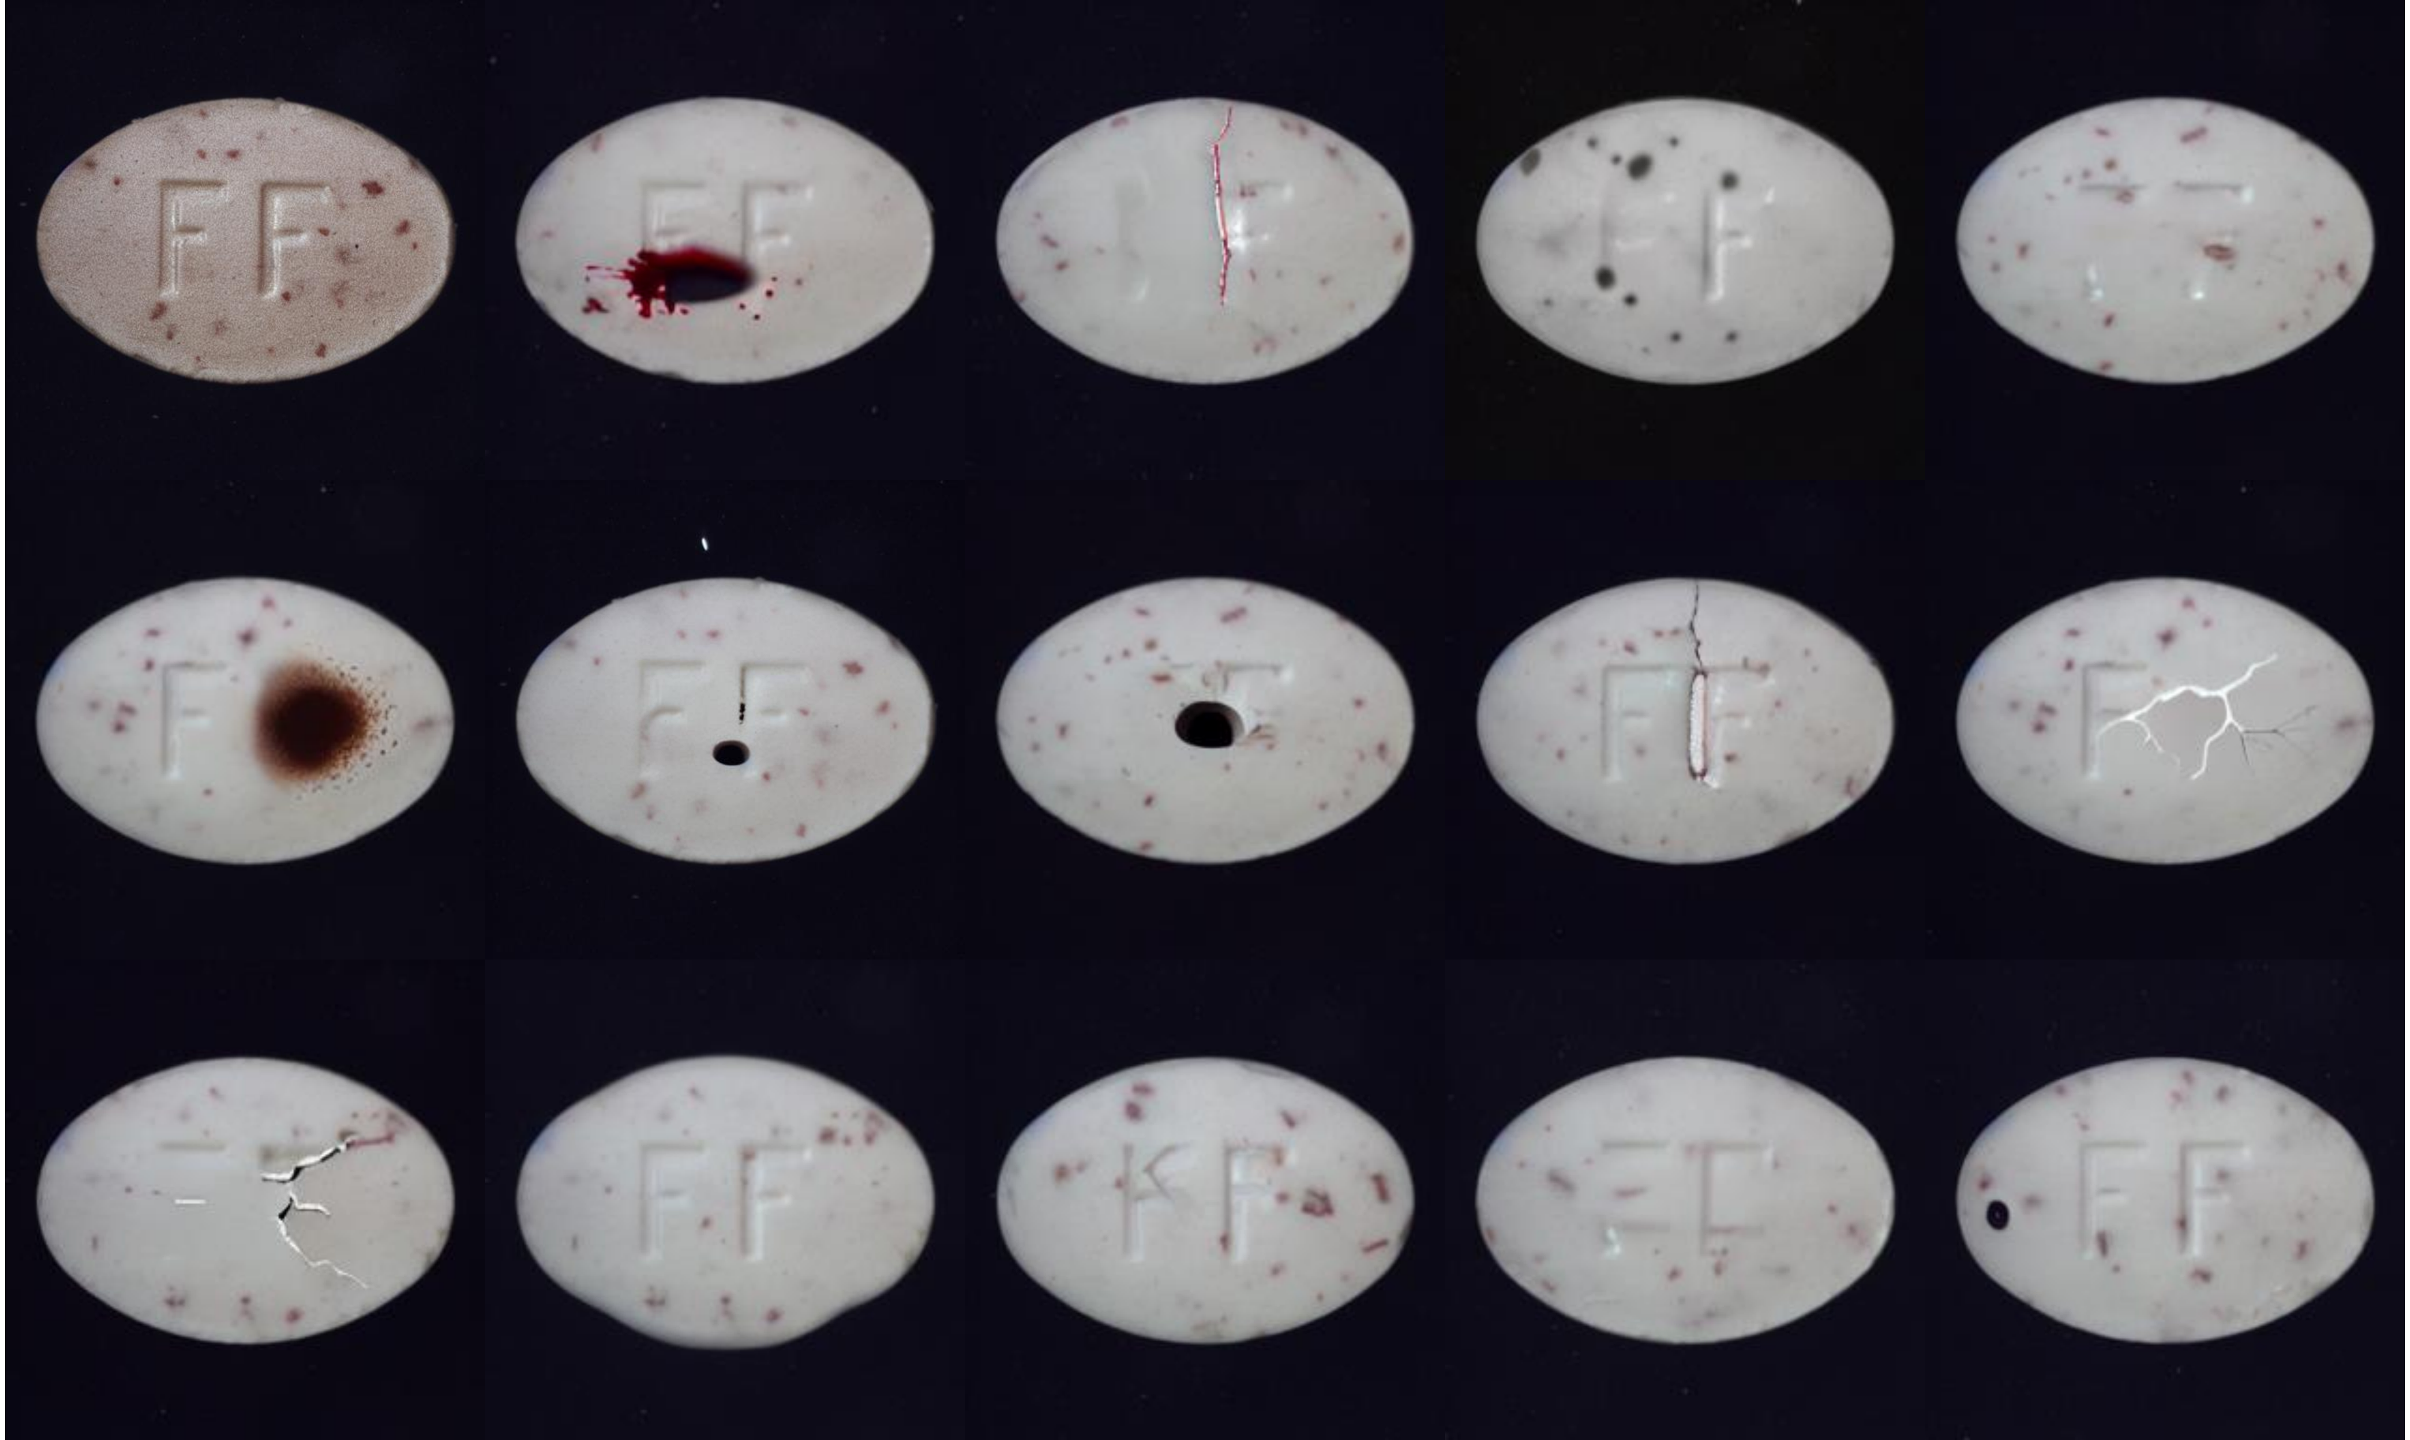

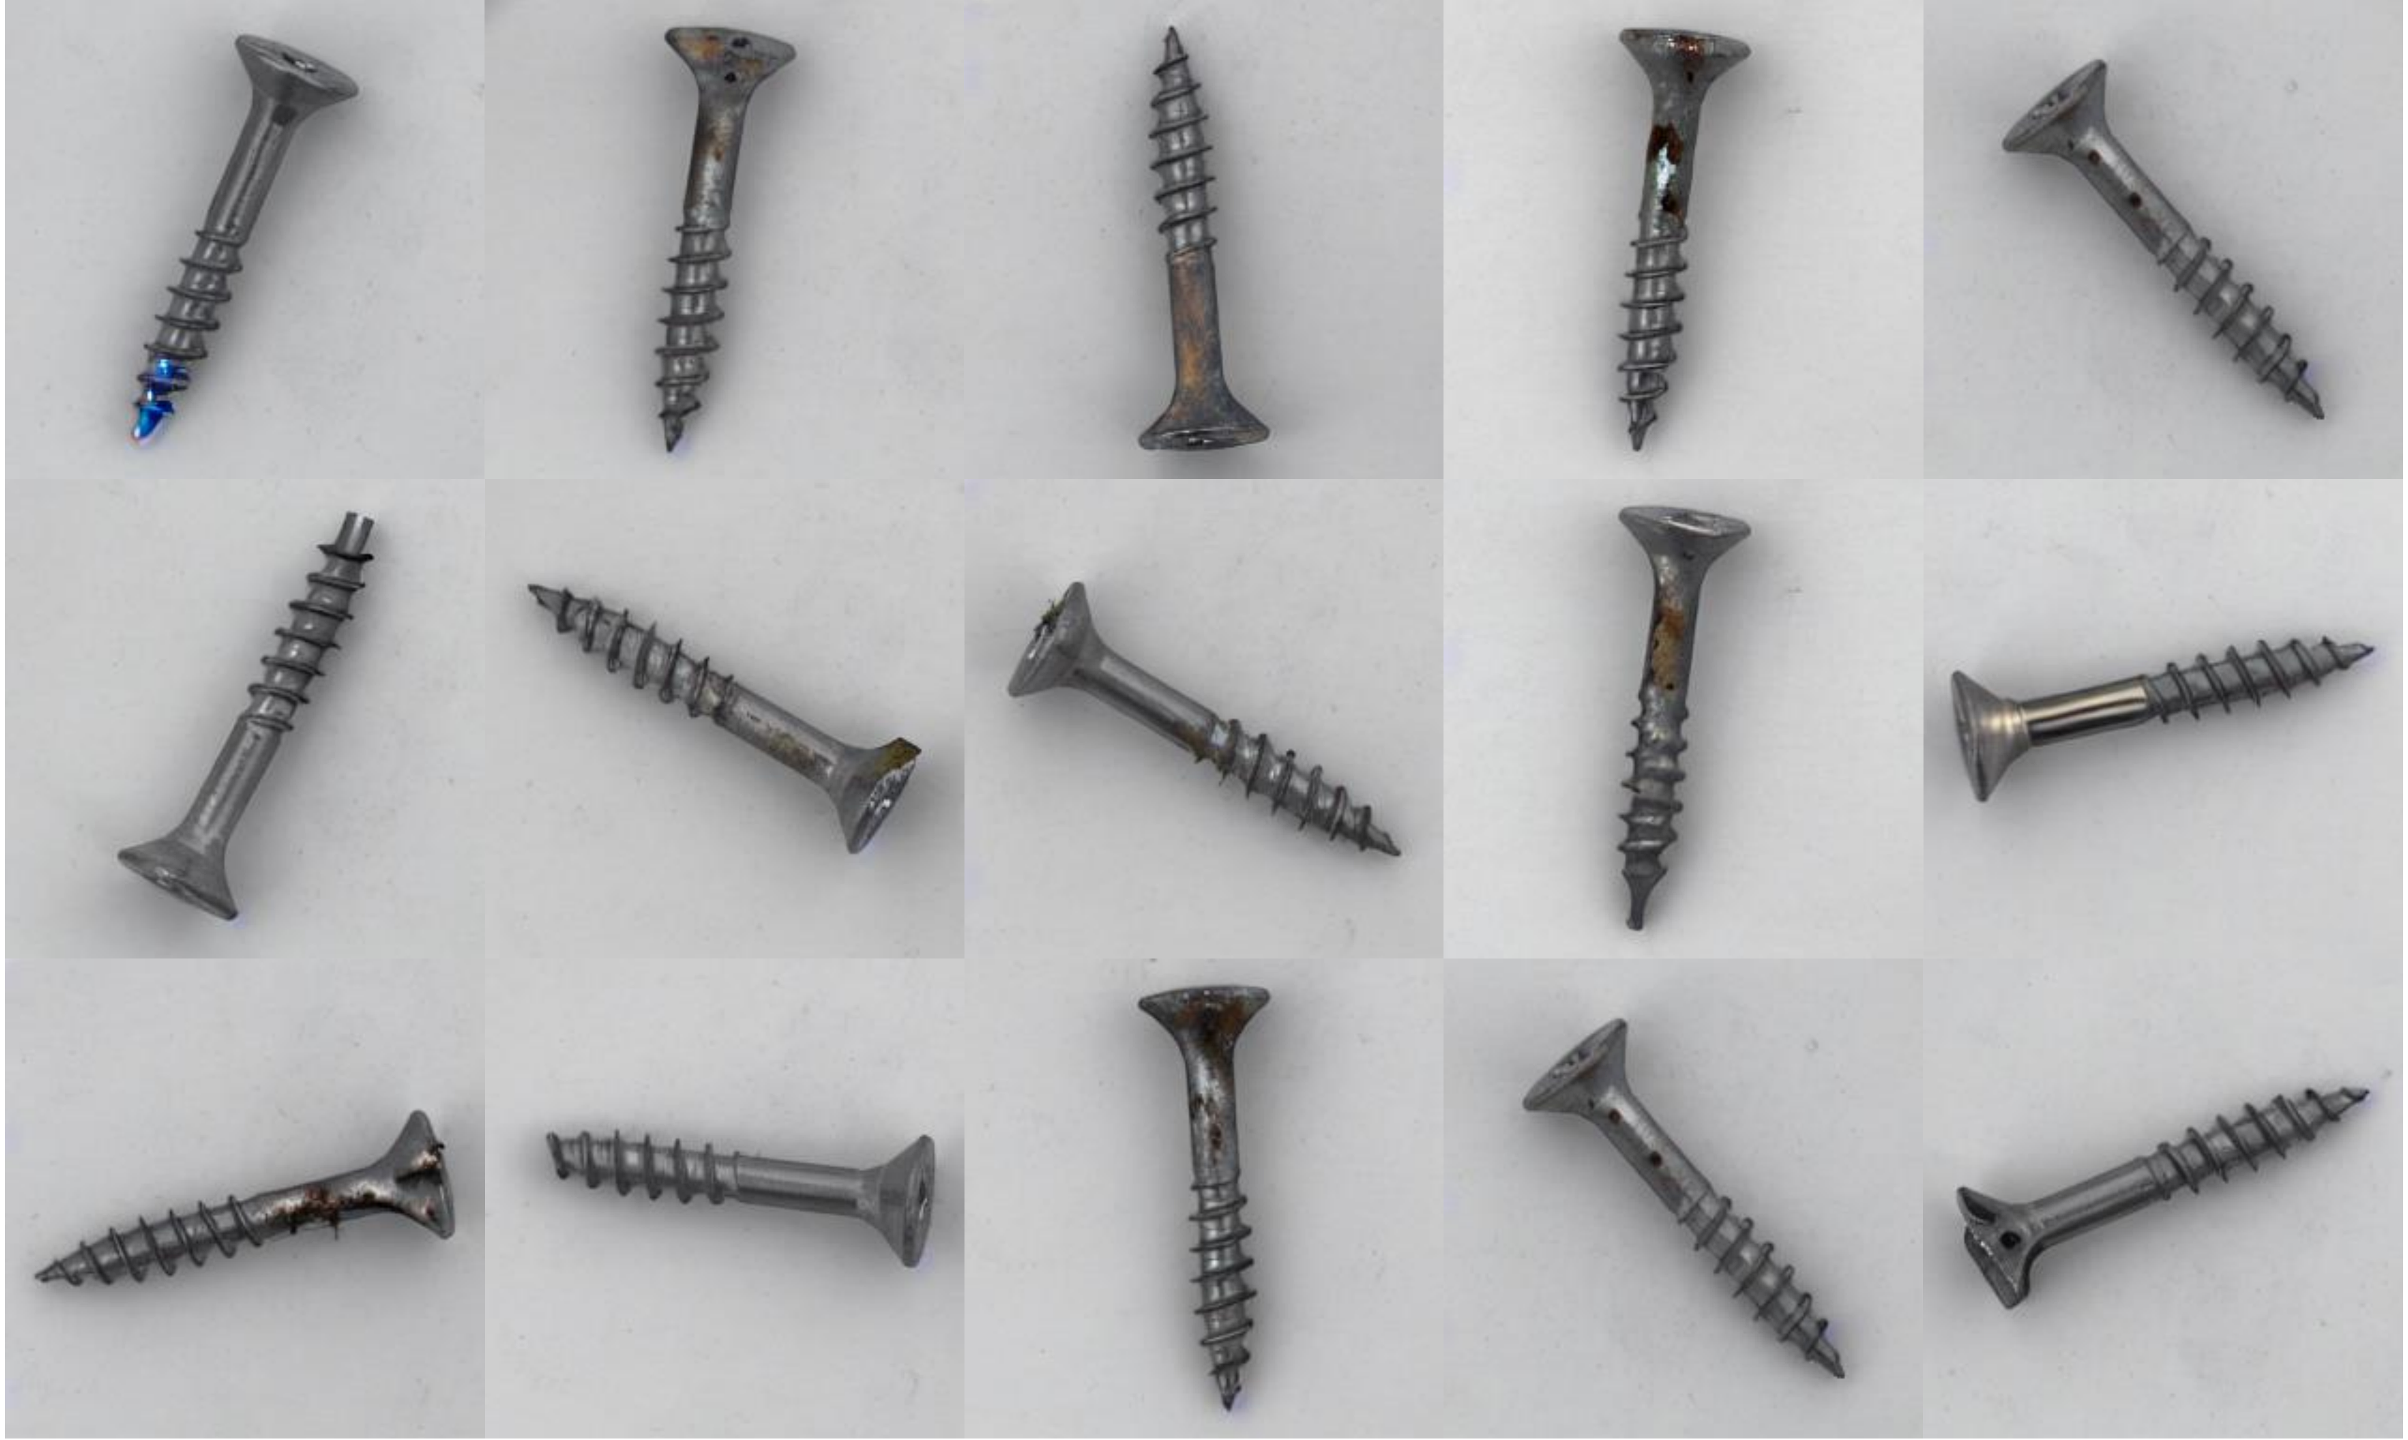

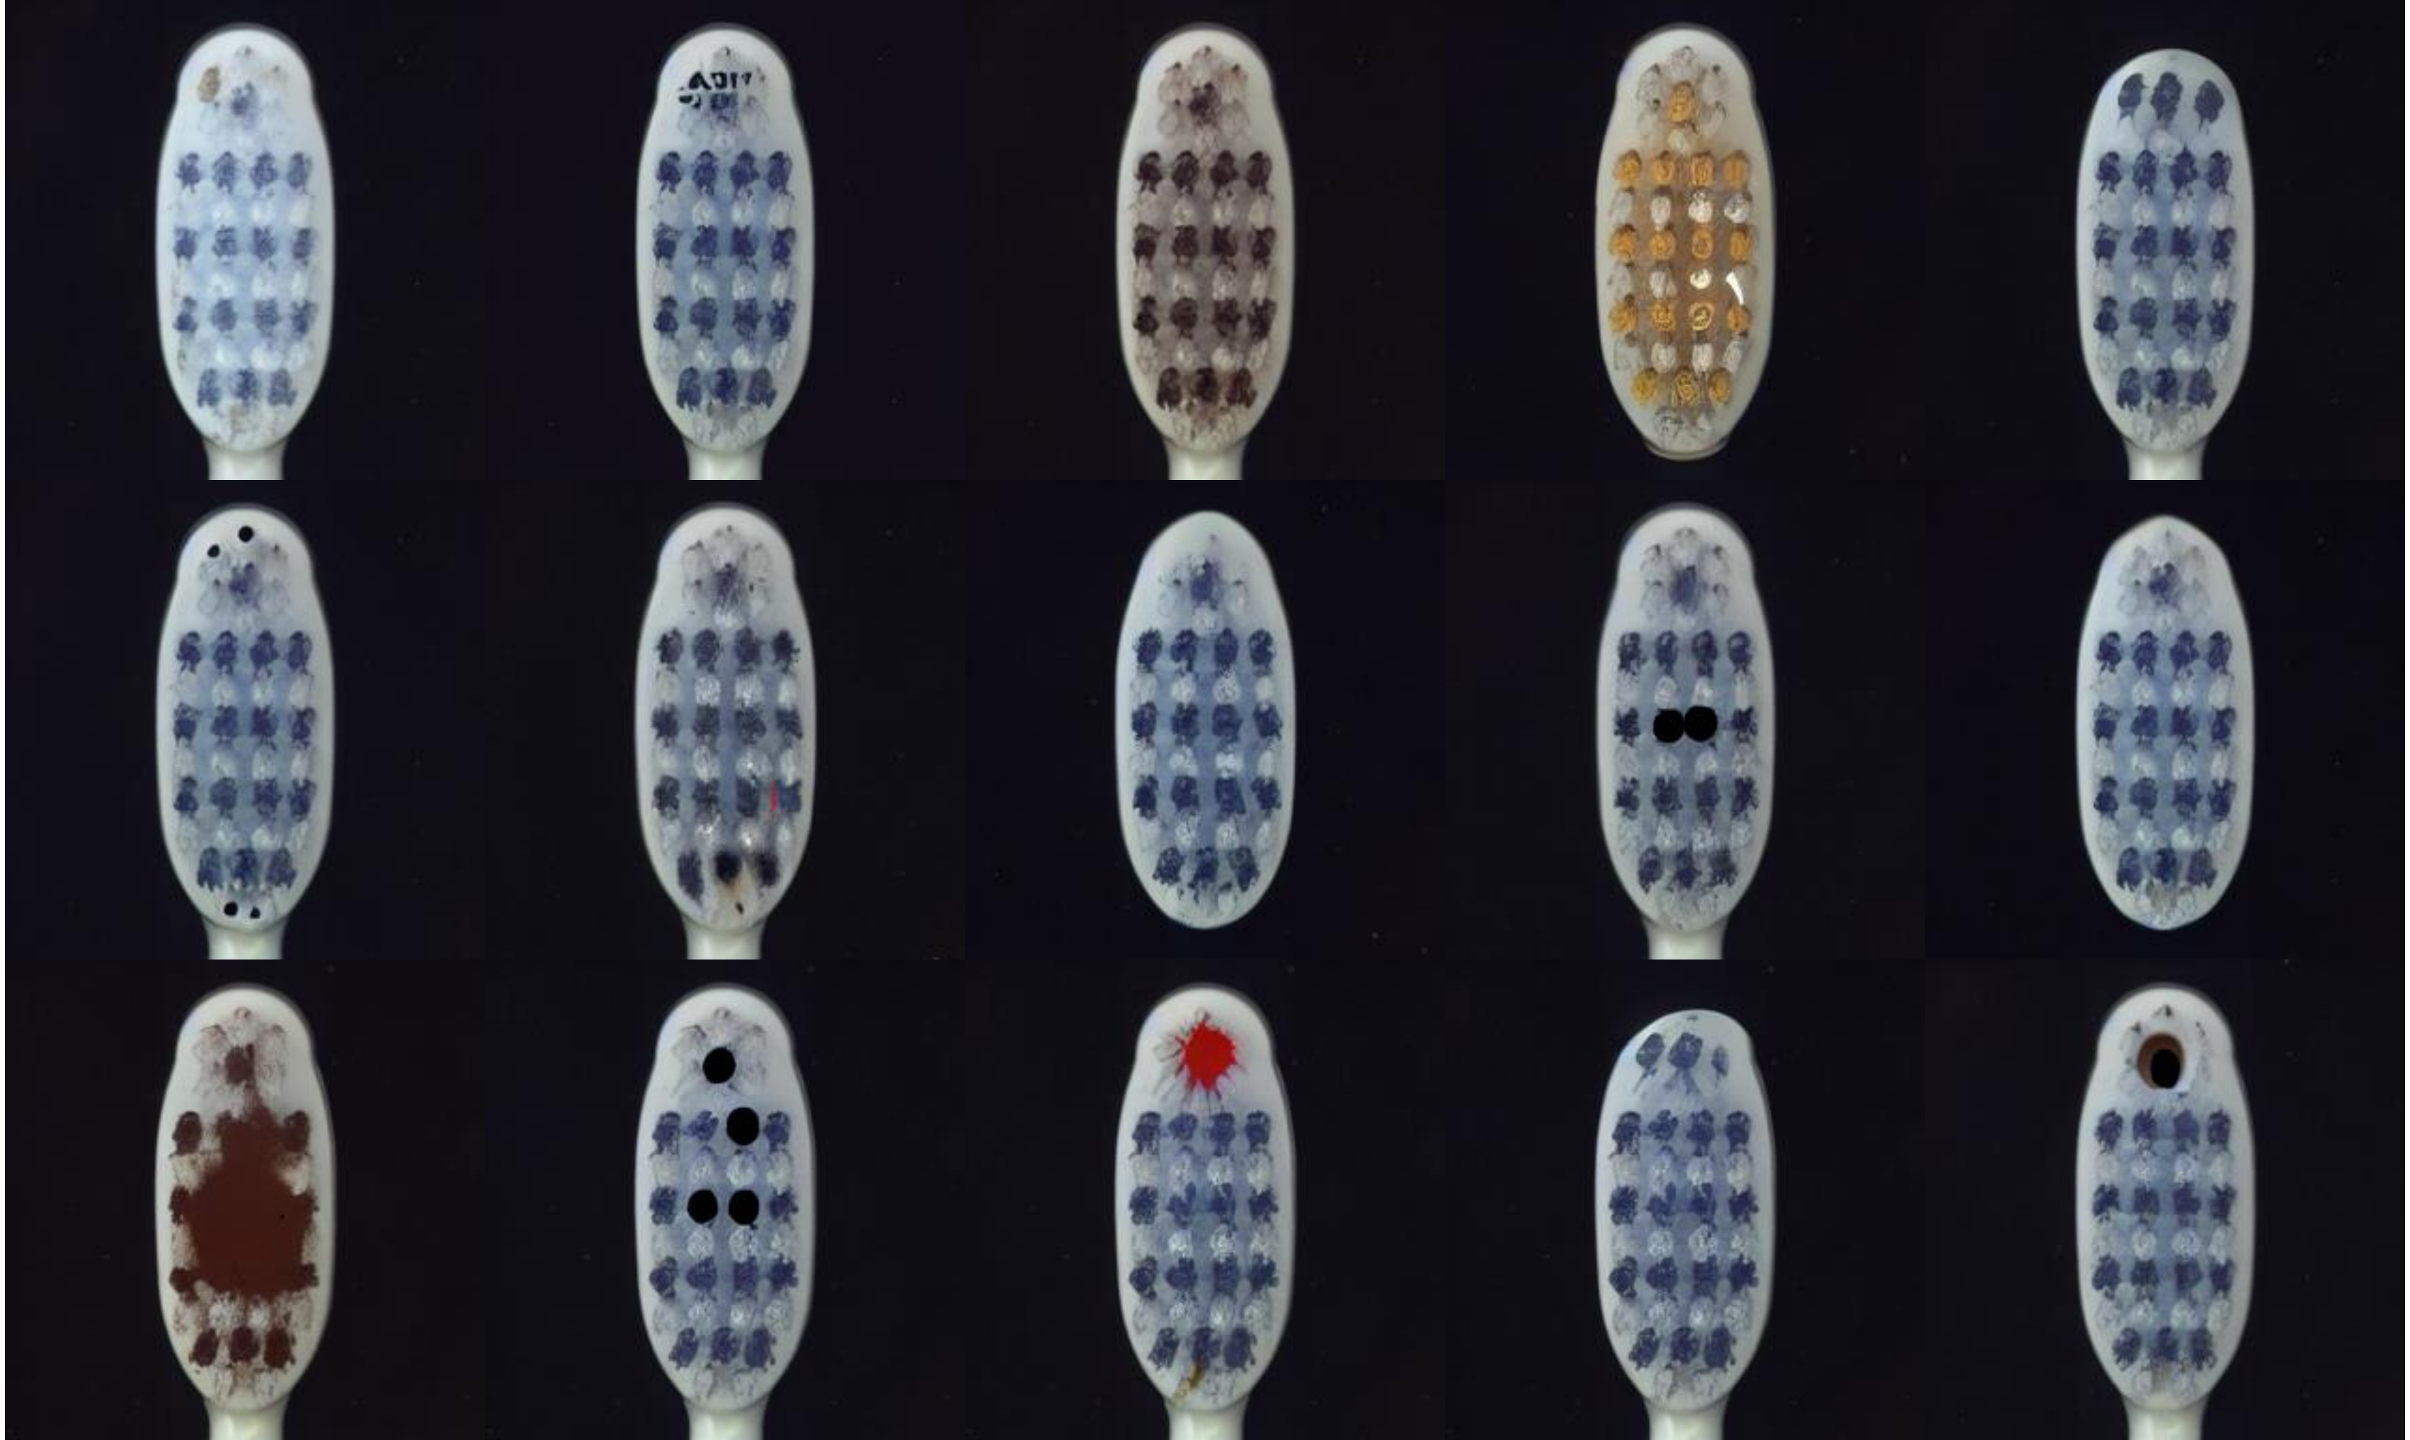

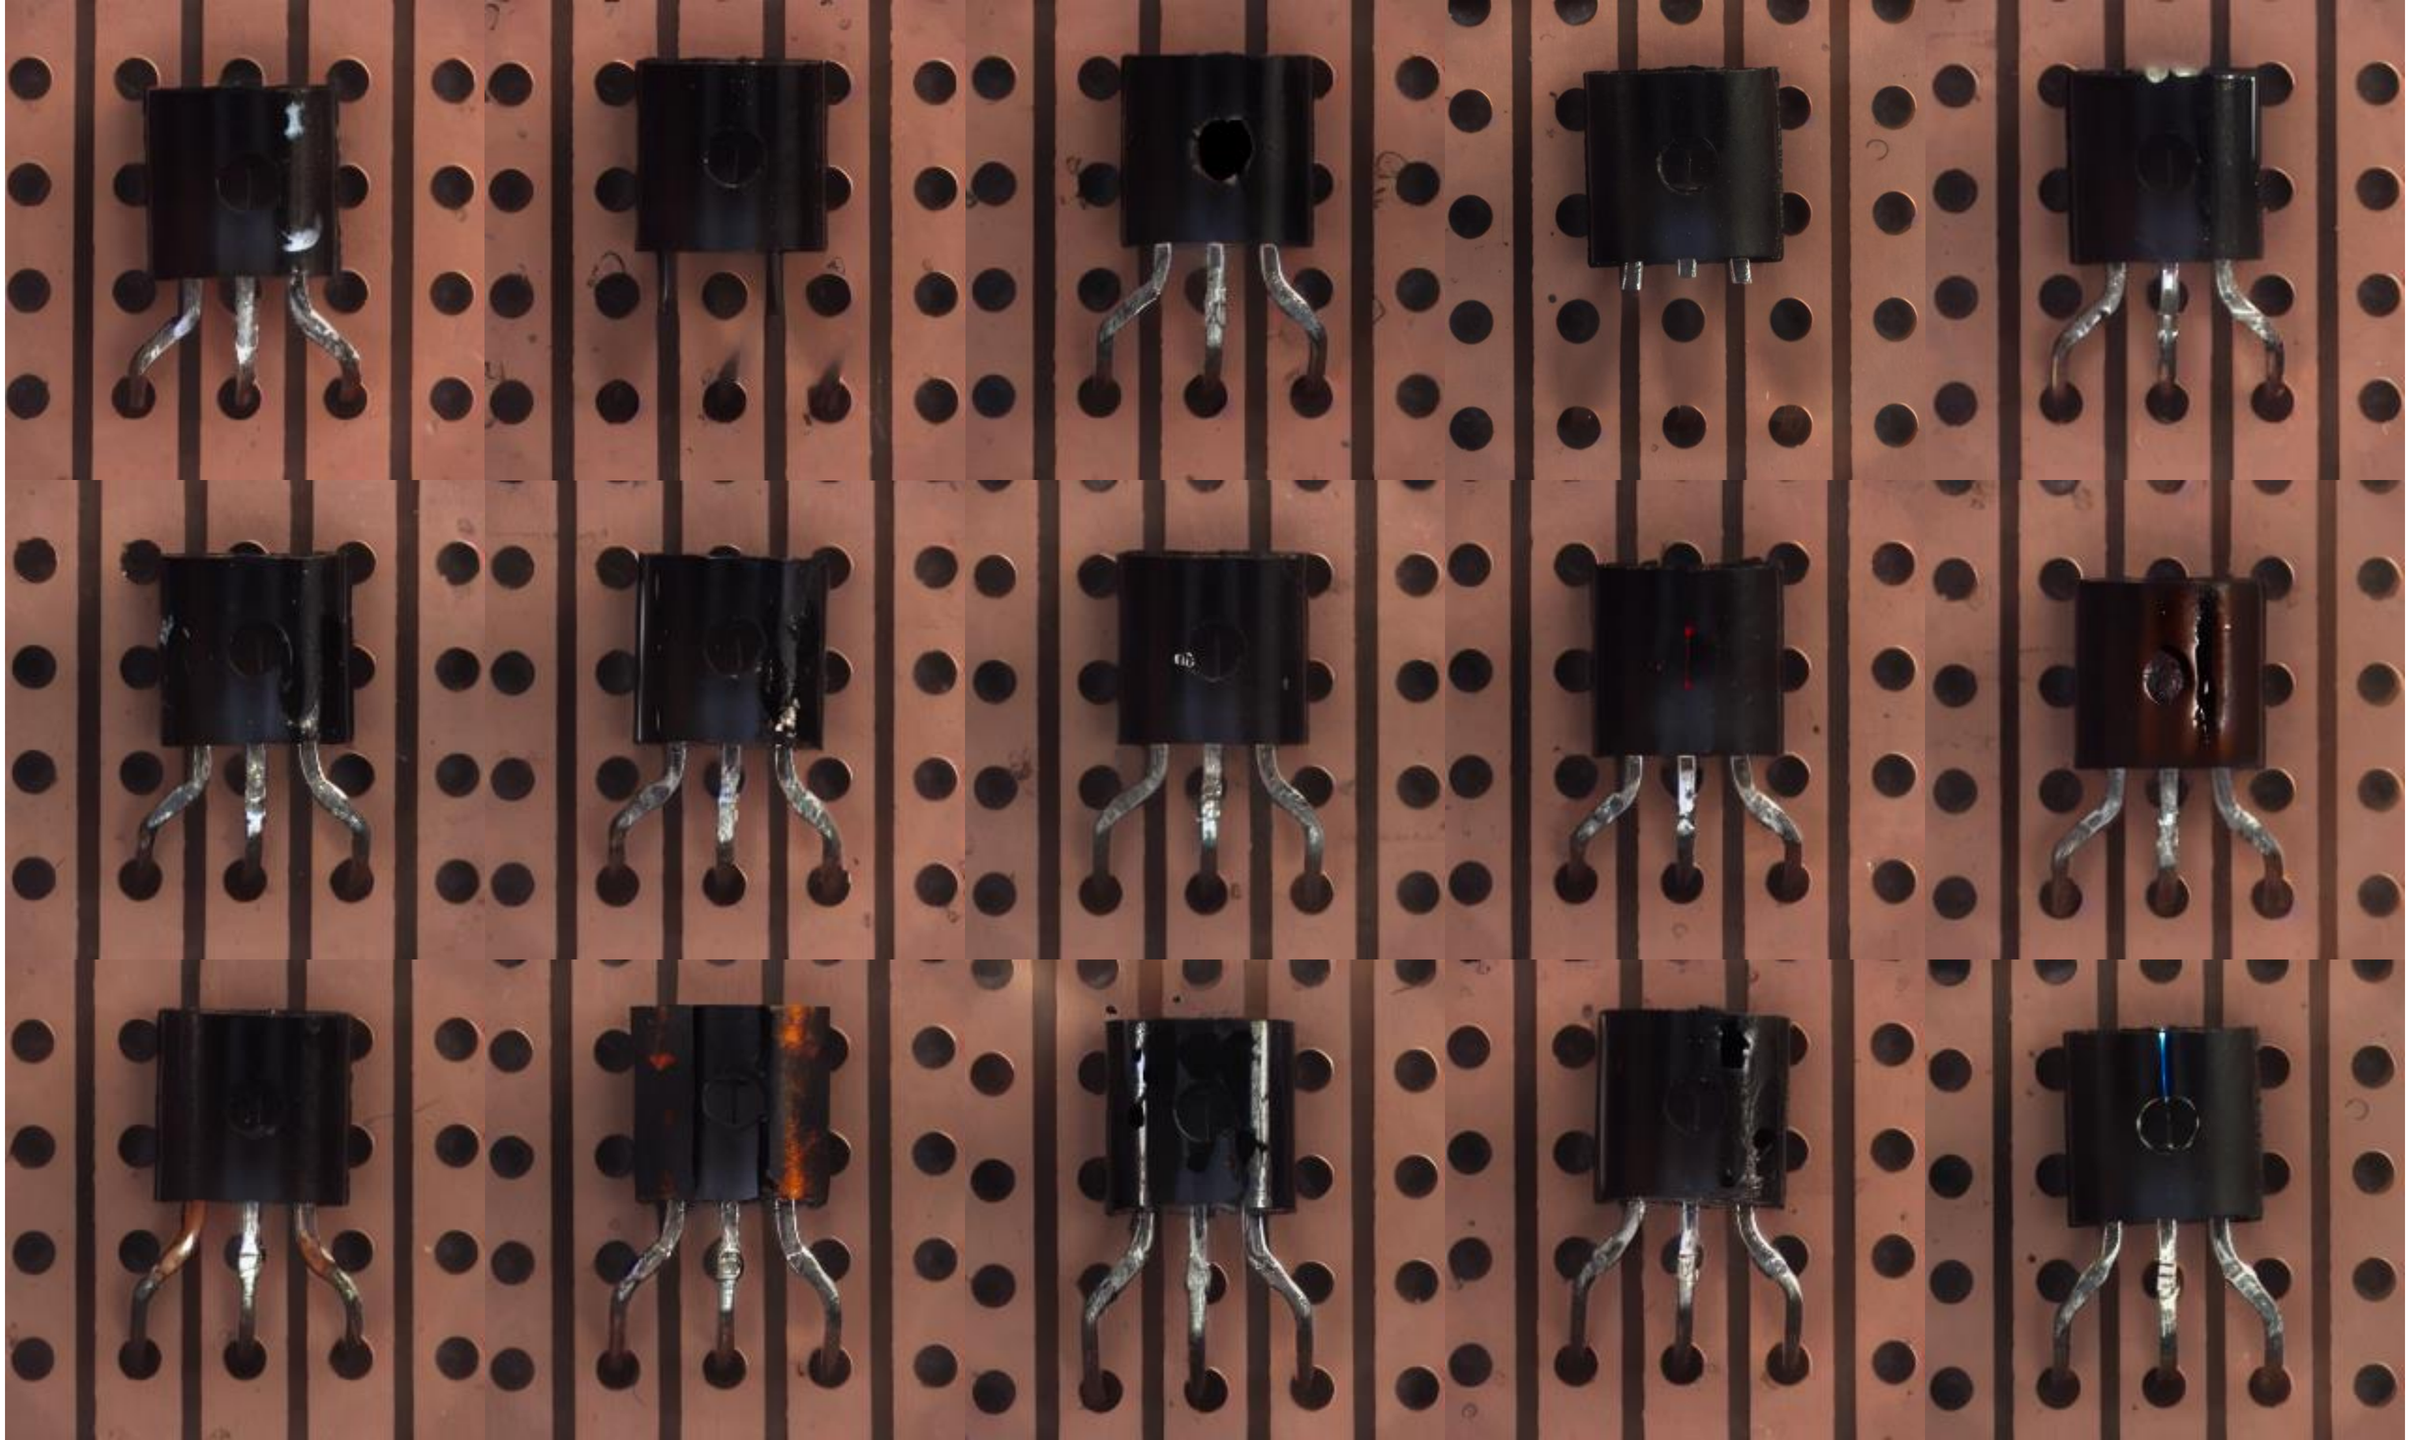

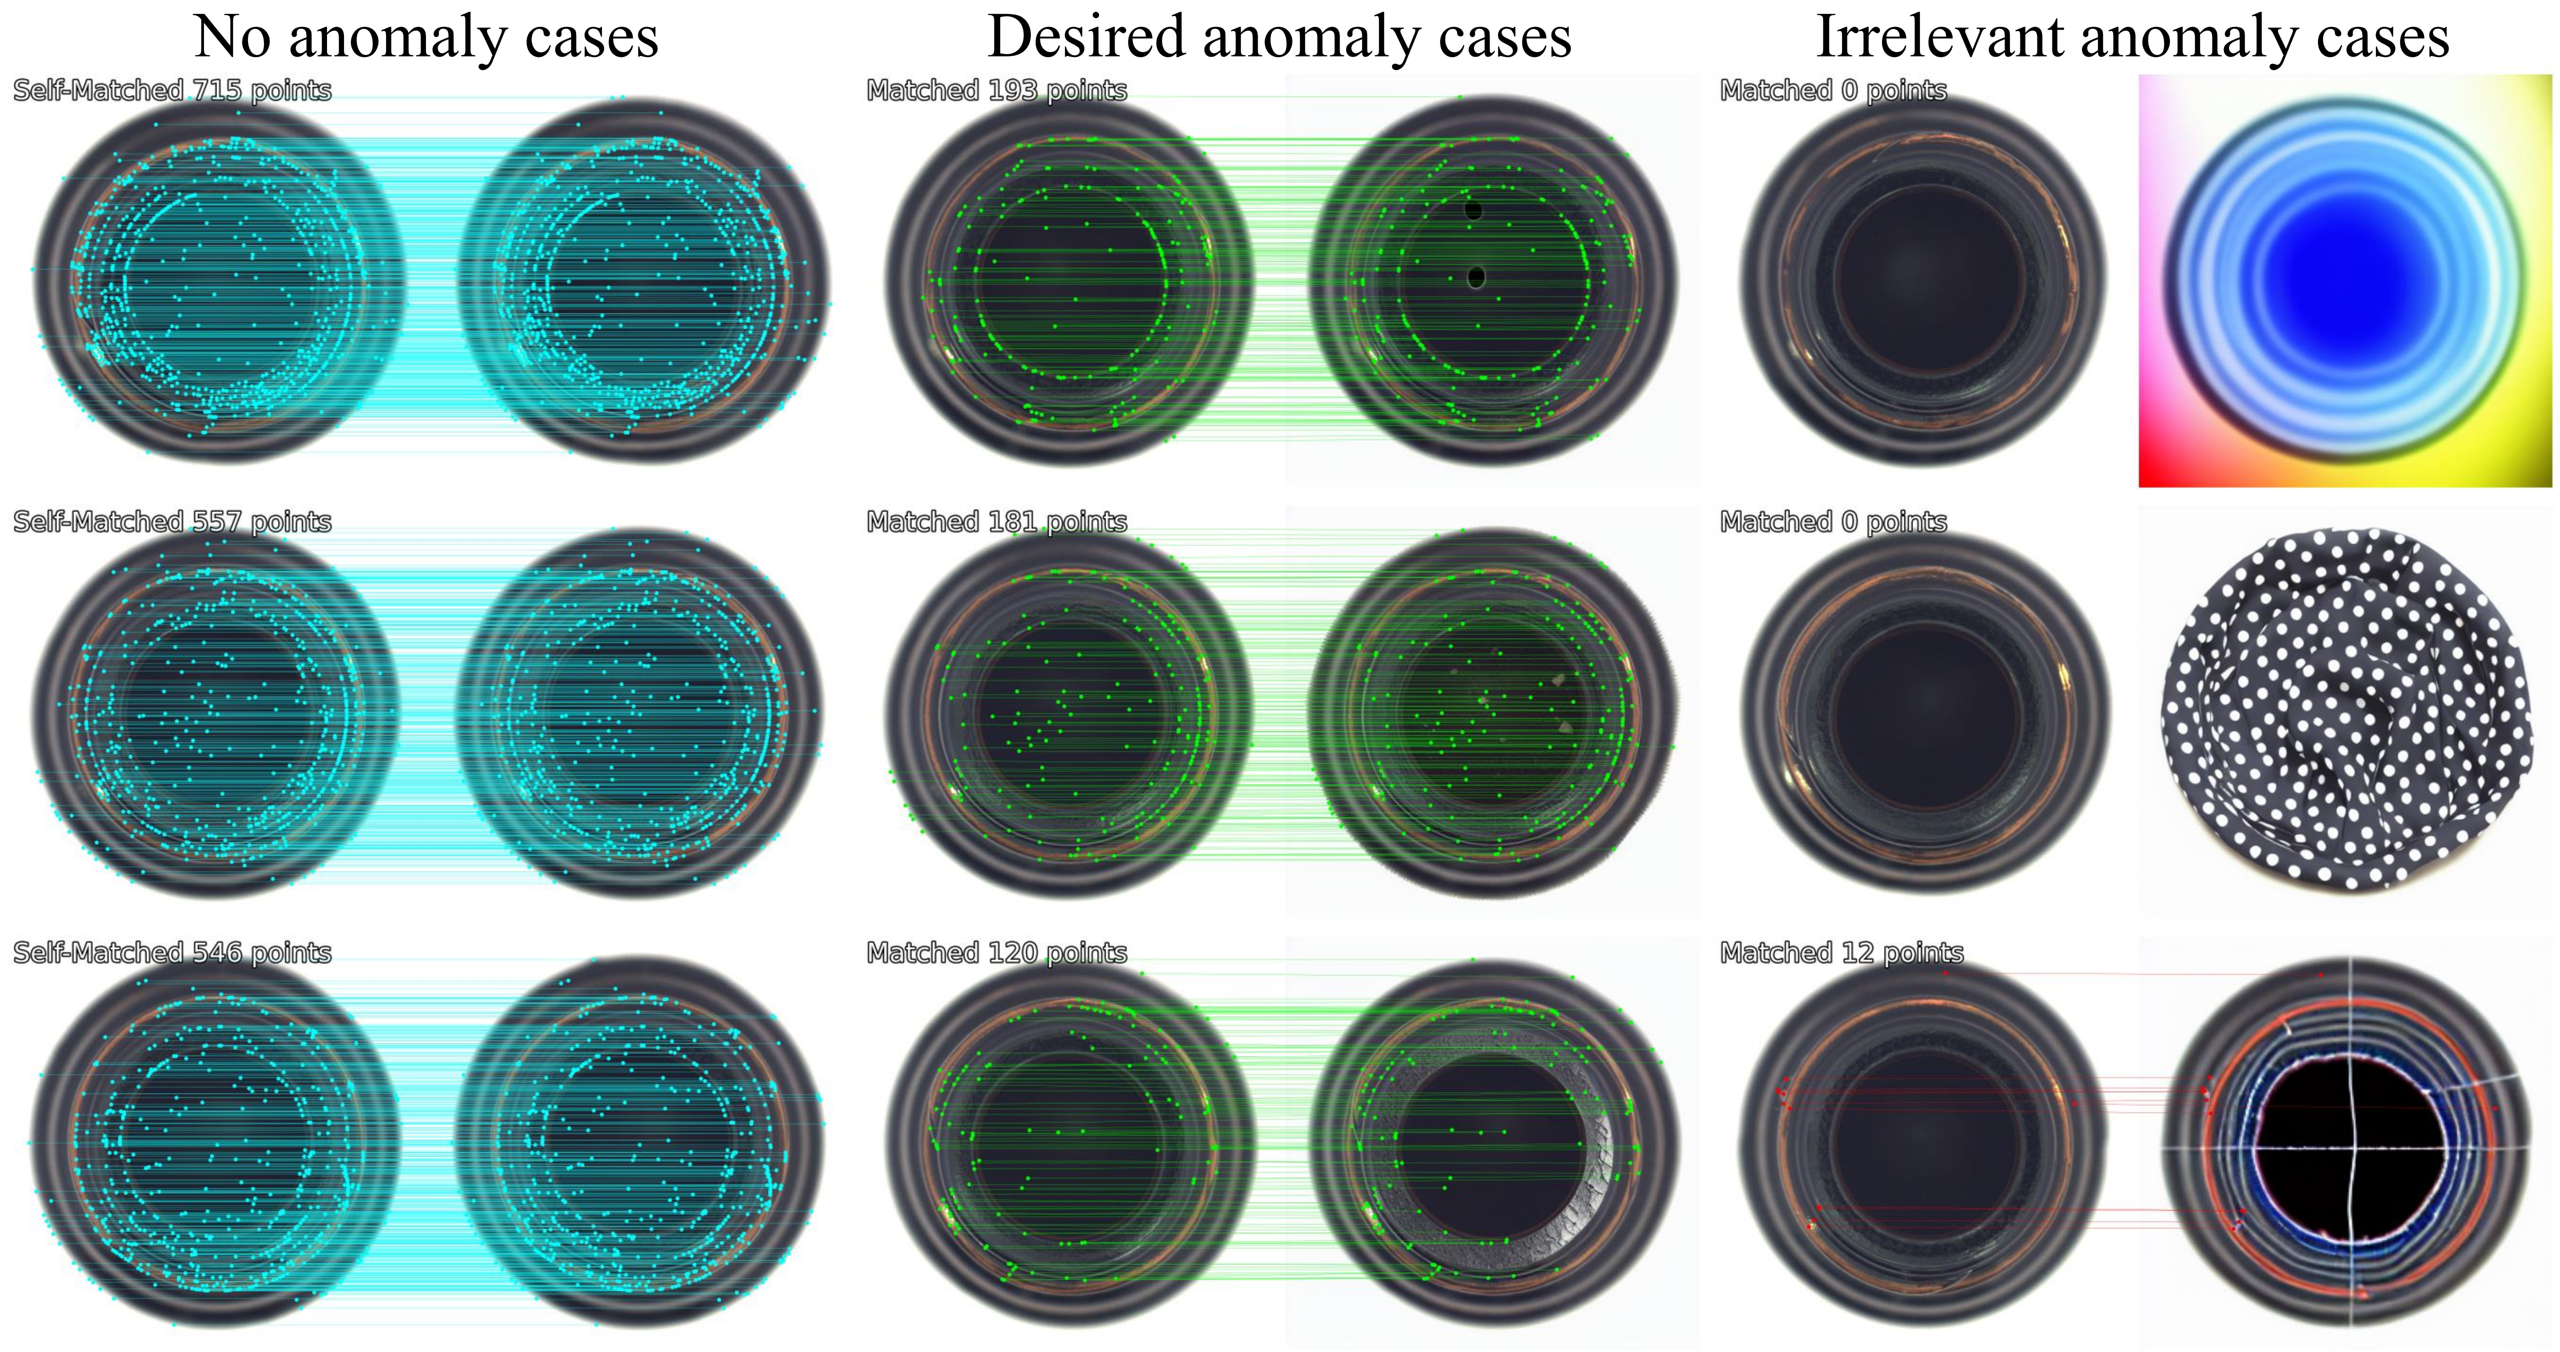
No anomaly cases
Desired anomaly cases
Irrelevant anomaly cases
Self-Matched 715 points
Matched 193 points
Matched 0 points
Self-Matched 557 points
Matched 181 points
Matched 0 points
Self-Matched 546 points
Matched 120 points
Matched 12 points

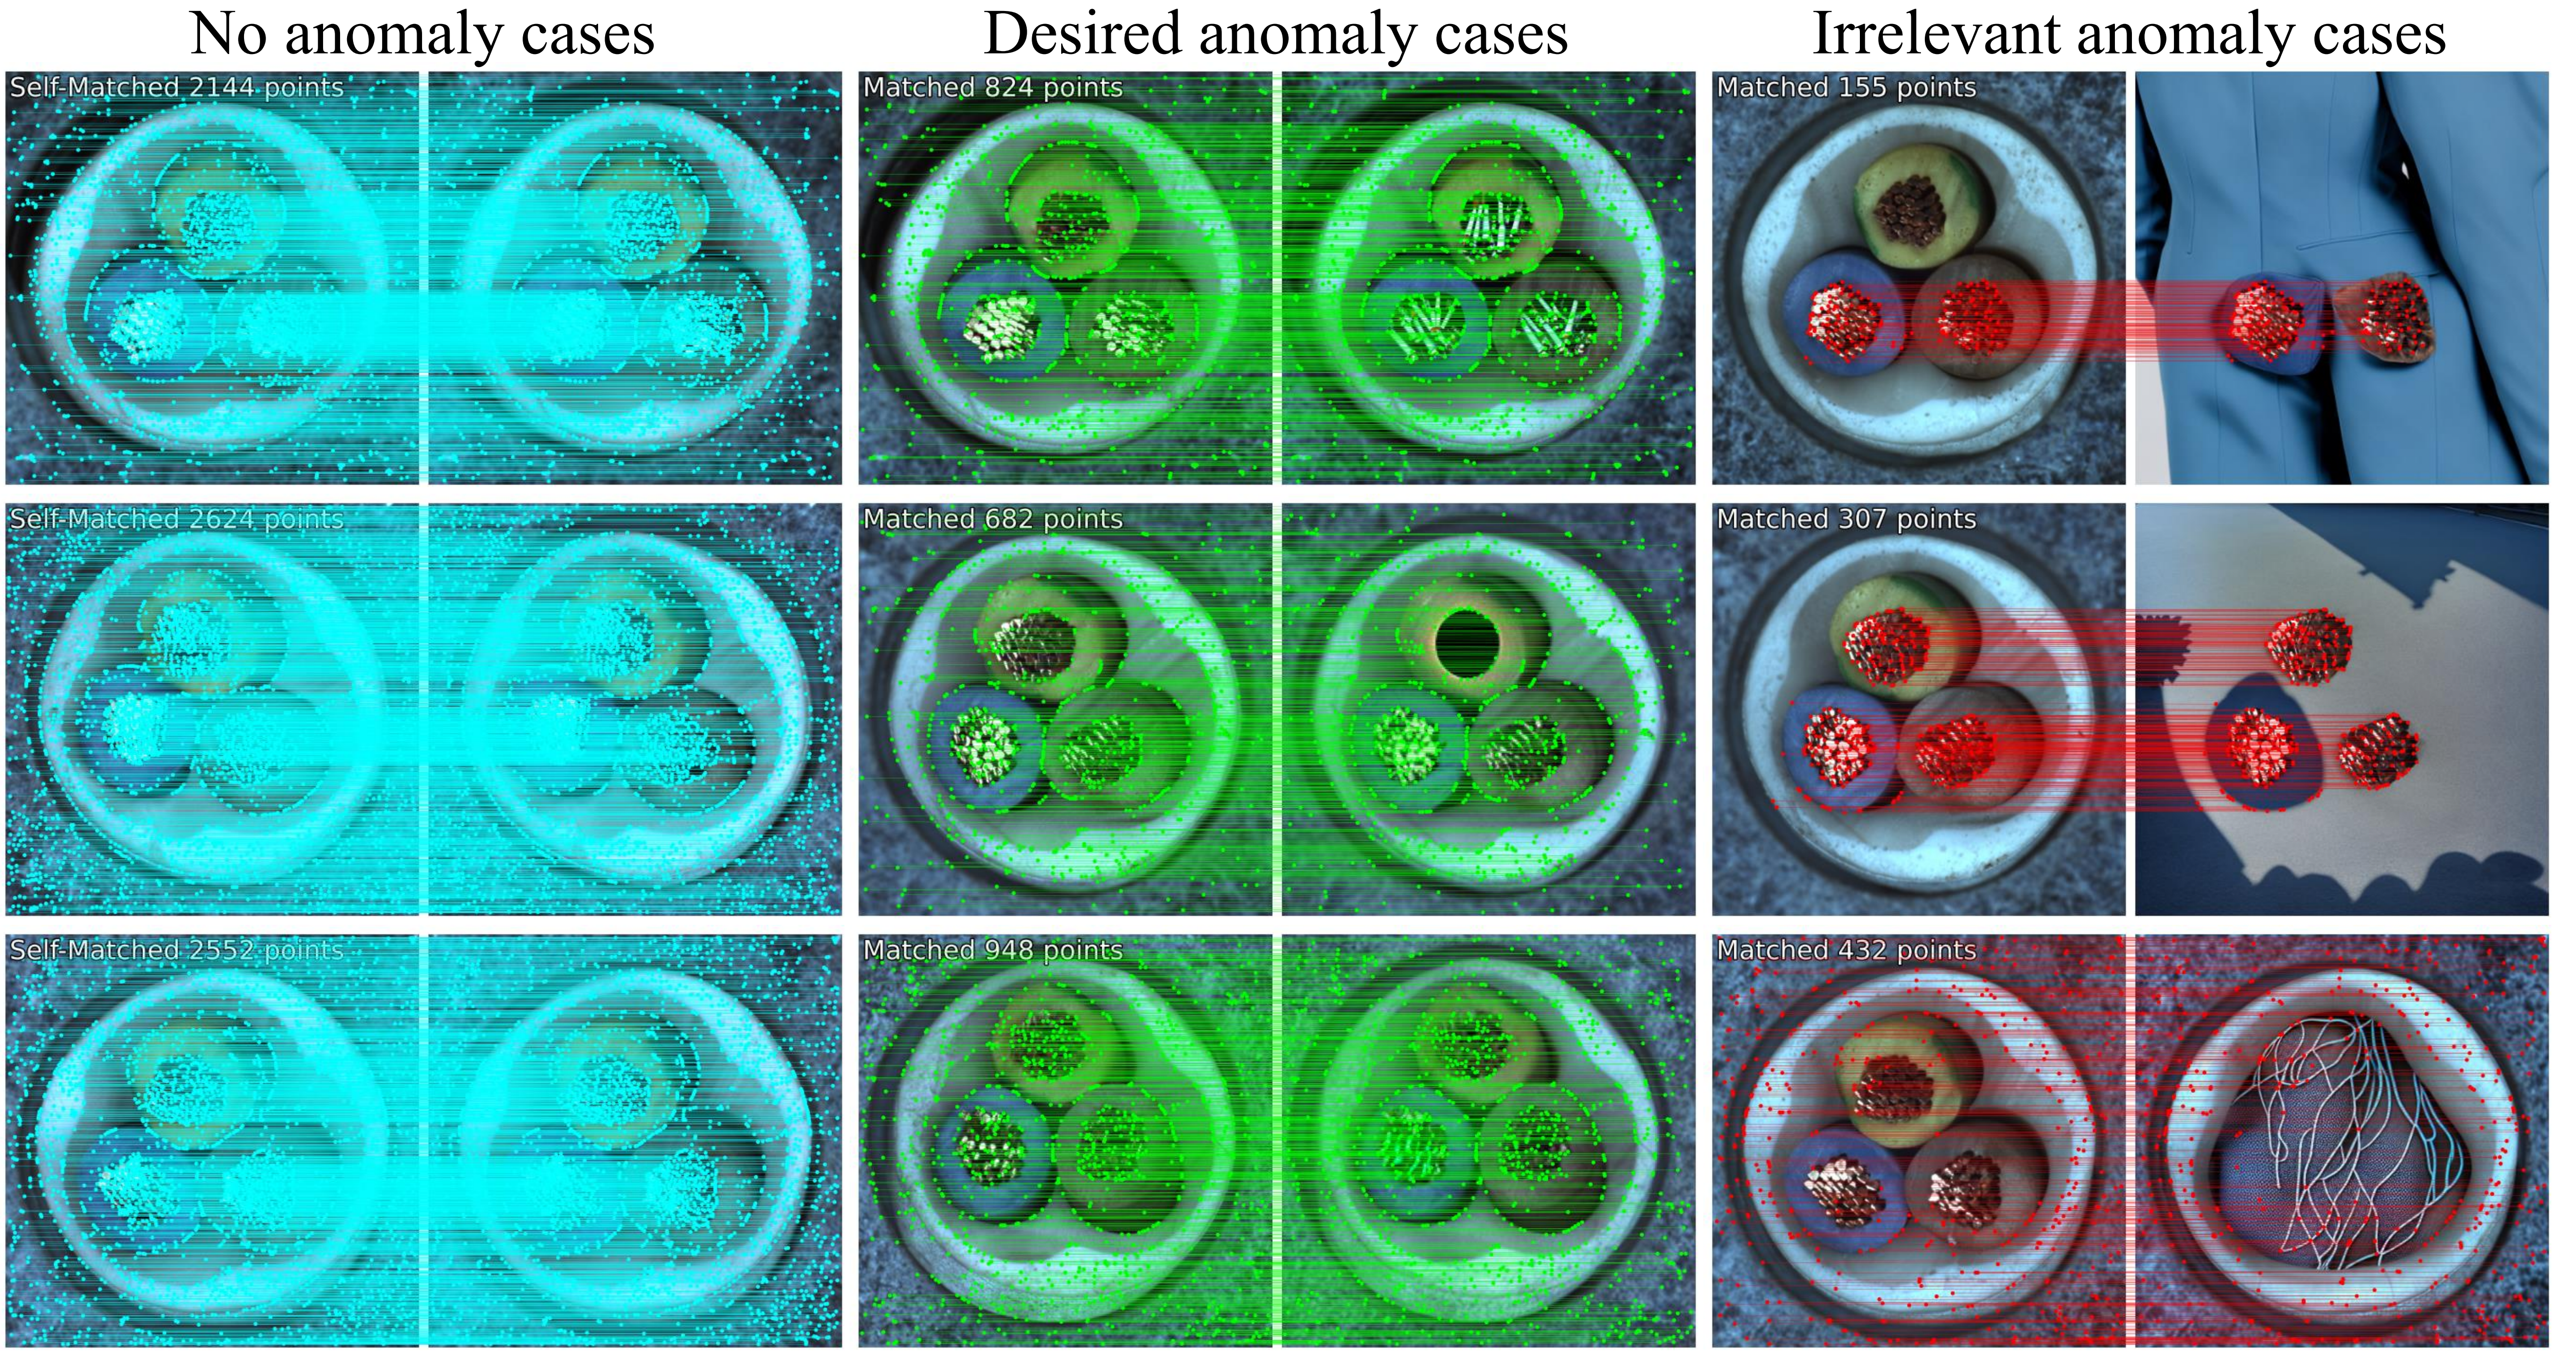
No anomaly cases
Desired anomaly cases
Irrelevant anomaly cases
Self-Matched 2144 points
Matched 824 points
Matched 155 points
Self-Matched 2624 points
Matched 682 points
Matched 307 points
Self-Matched 2552 points
Matched 948 points
Matched 432 points

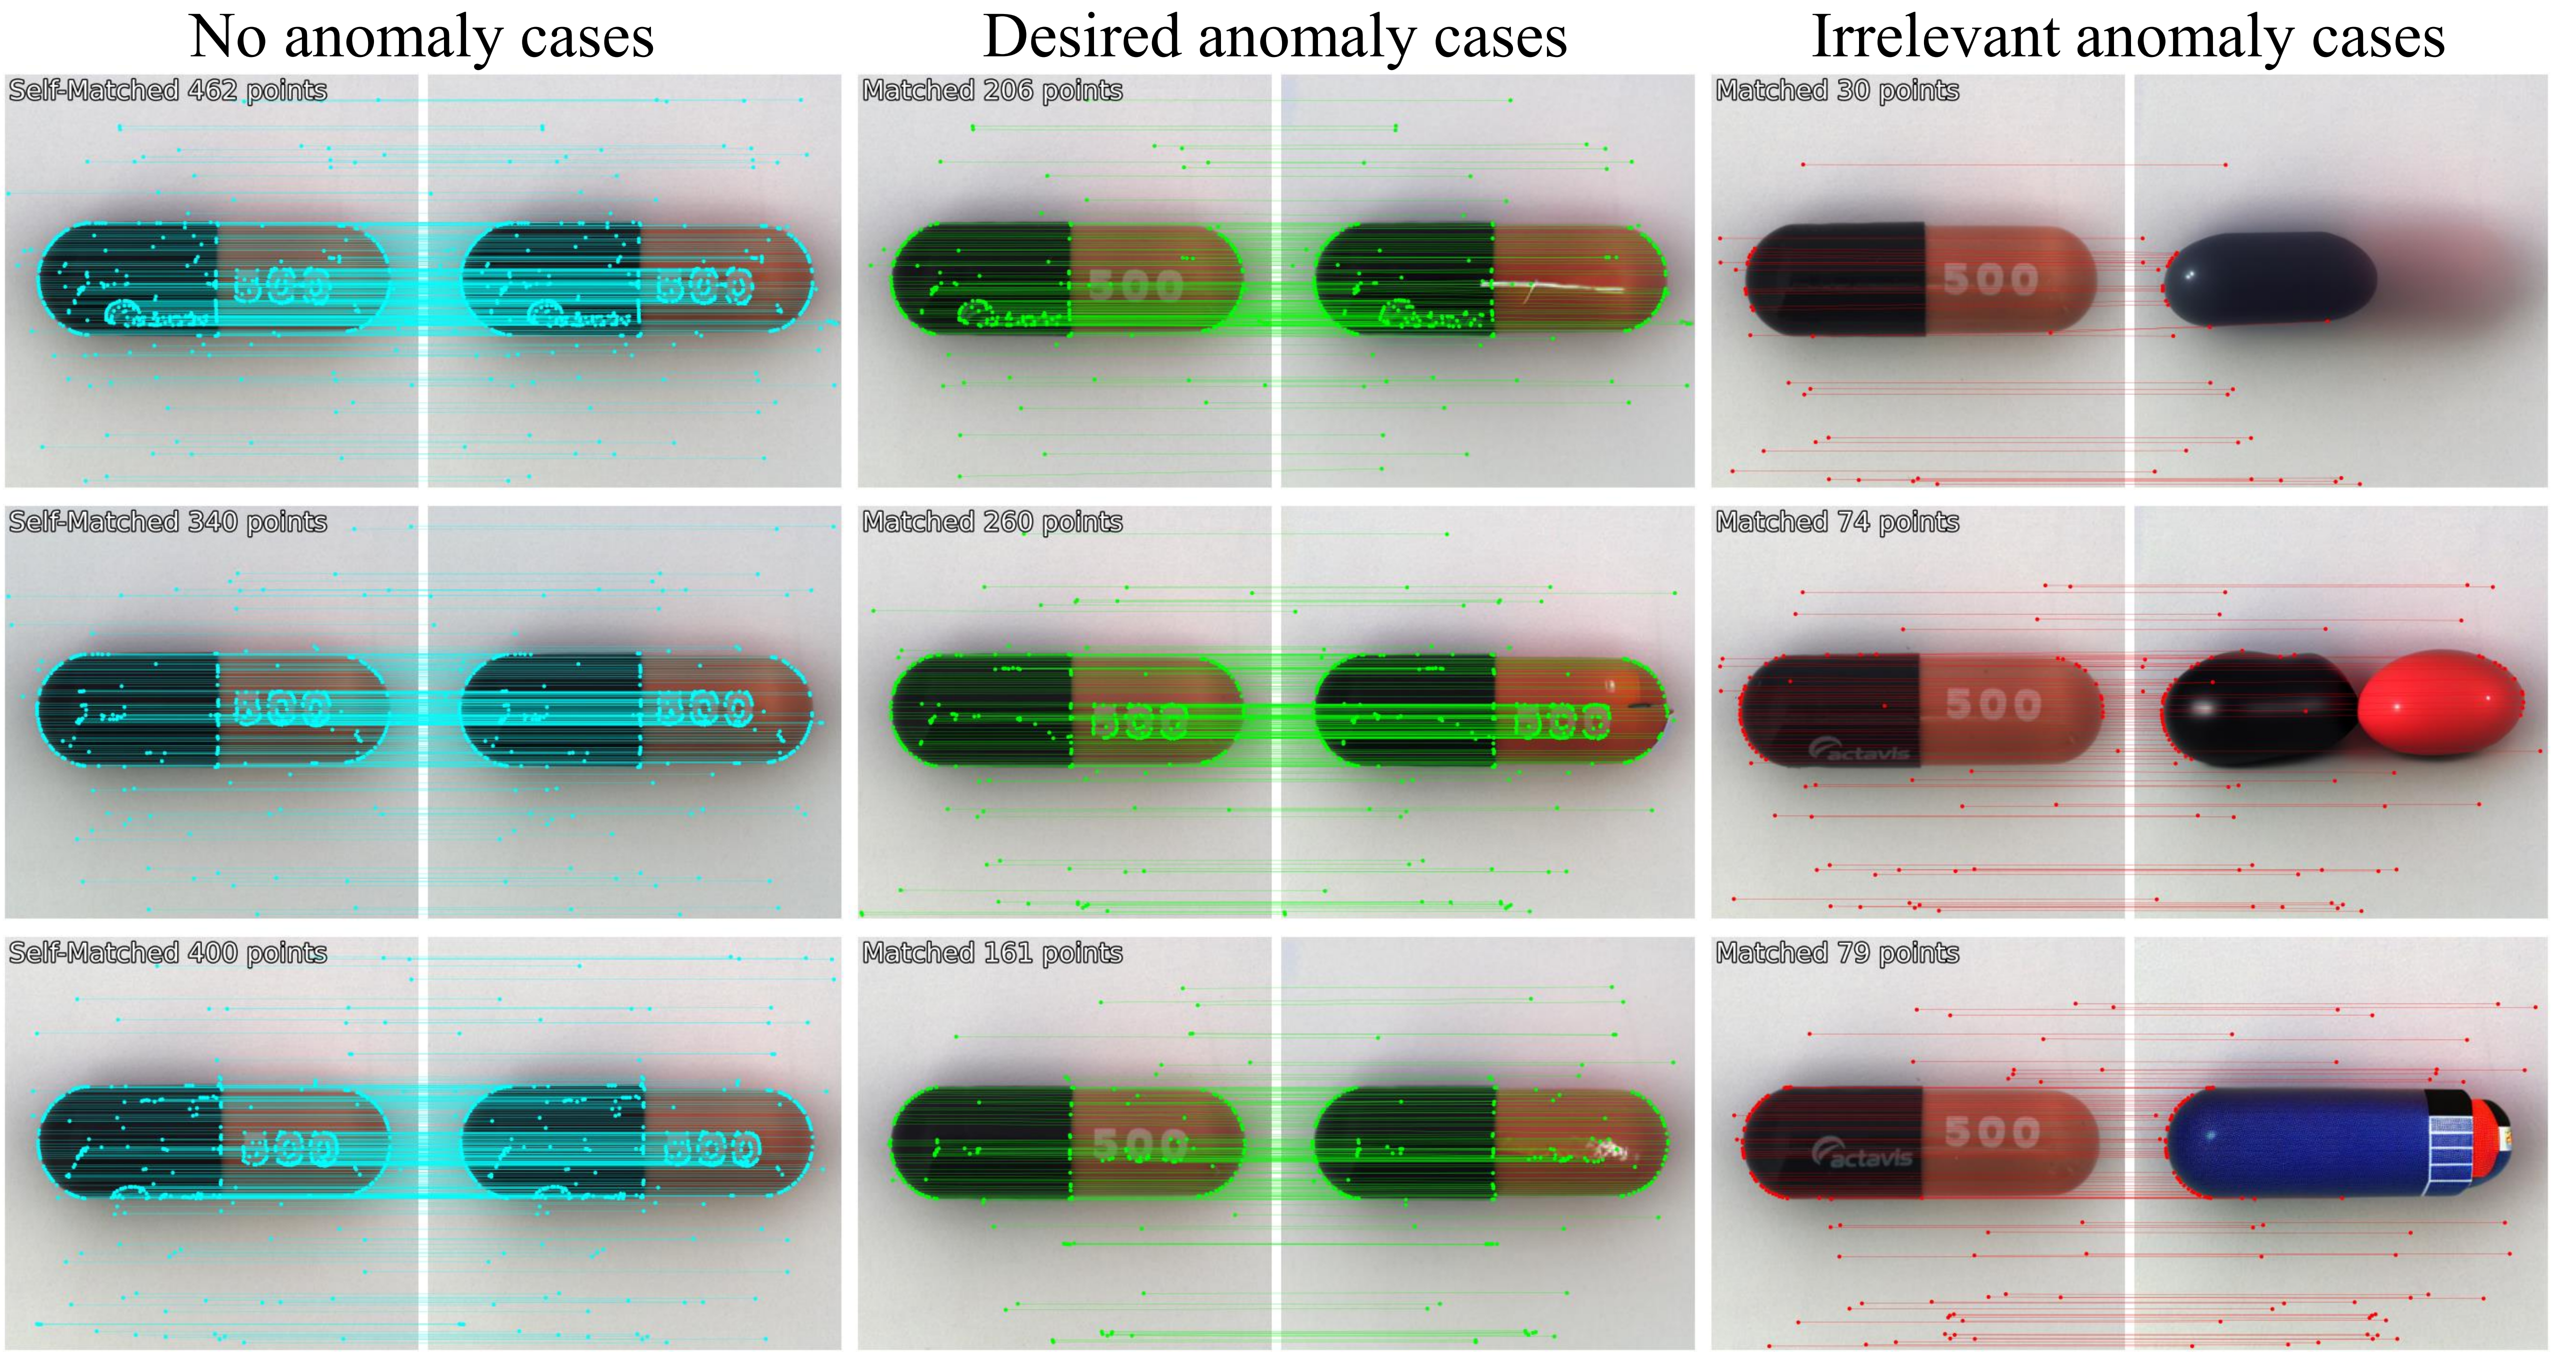
No anomaly cases
Desired anomaly cases
Irrelevant anomaly cases
Self-Matched 462 points
Matched 206 points
Matched 30 points
Self-Matched 340 points
Matched 260 points
Matched 74 points
Self-Matched 400 points
Matched 161 points
Matched 79 points

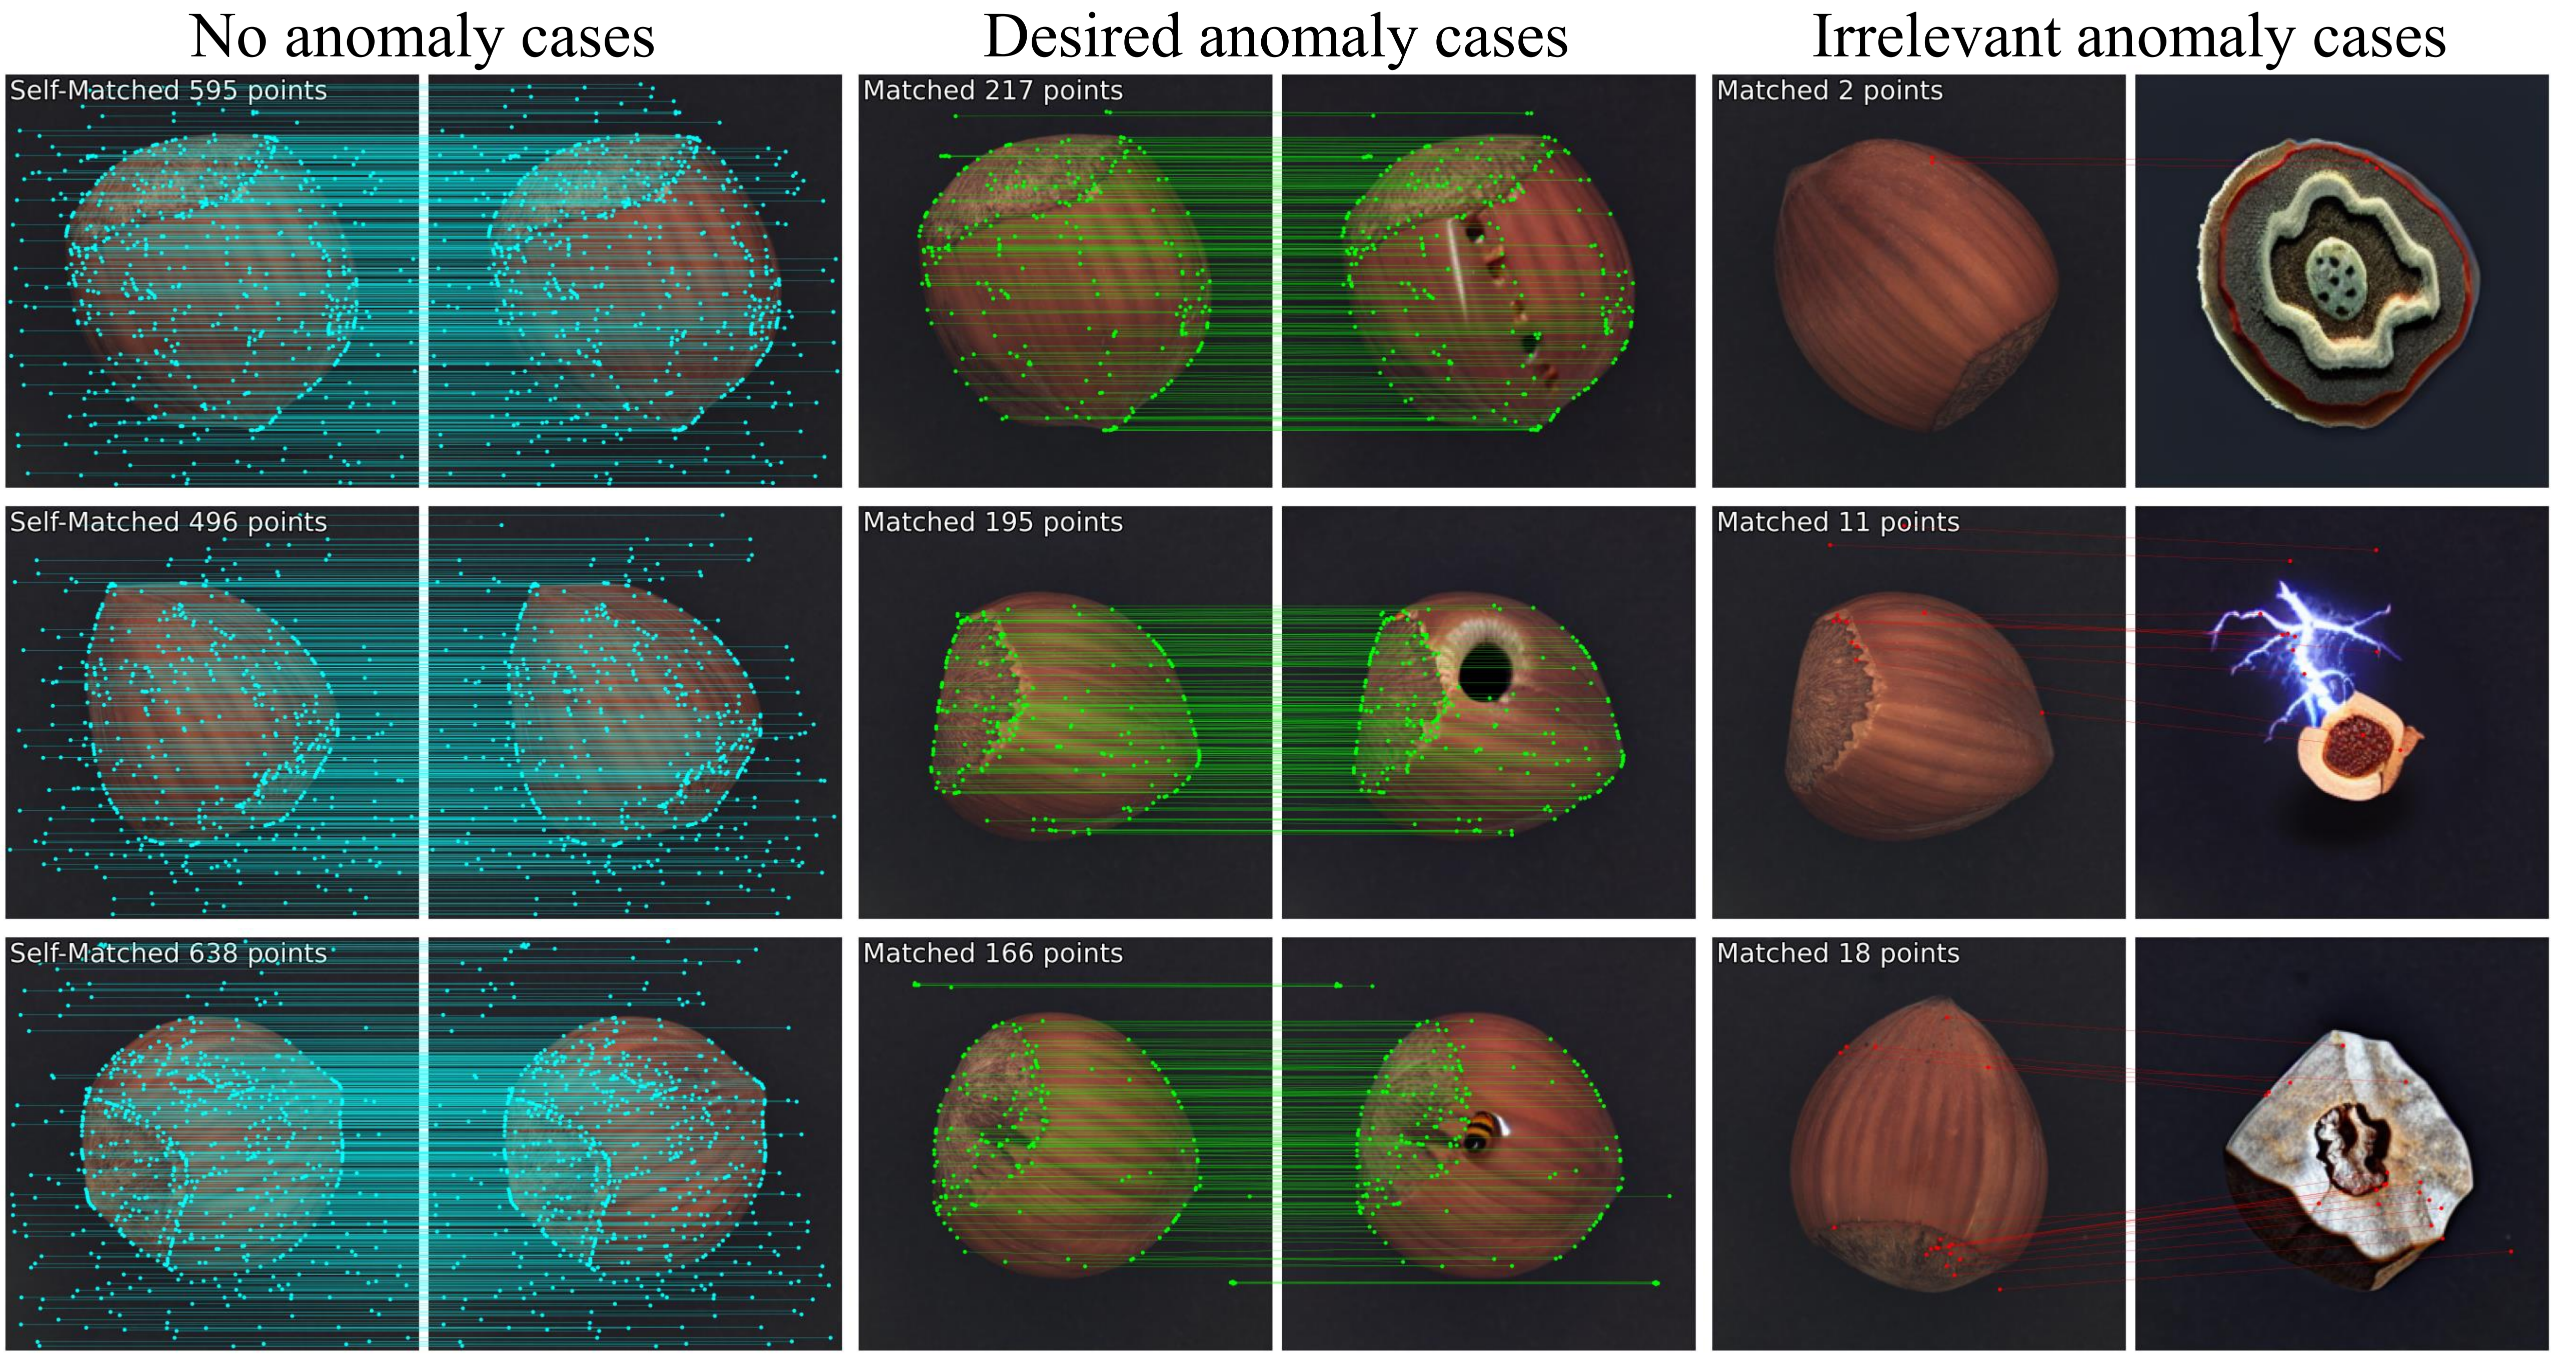

No anomaly cases
Desired anomaly cases
Irrelevant anomaly cases
Self-Matched 595 points
Matched 217 points
Matched 2 points
Self-Matched 496 points
Matched 195 points
Matched 11 points
Self-Matched 638 points
Matched 166 points
Matched 18 points

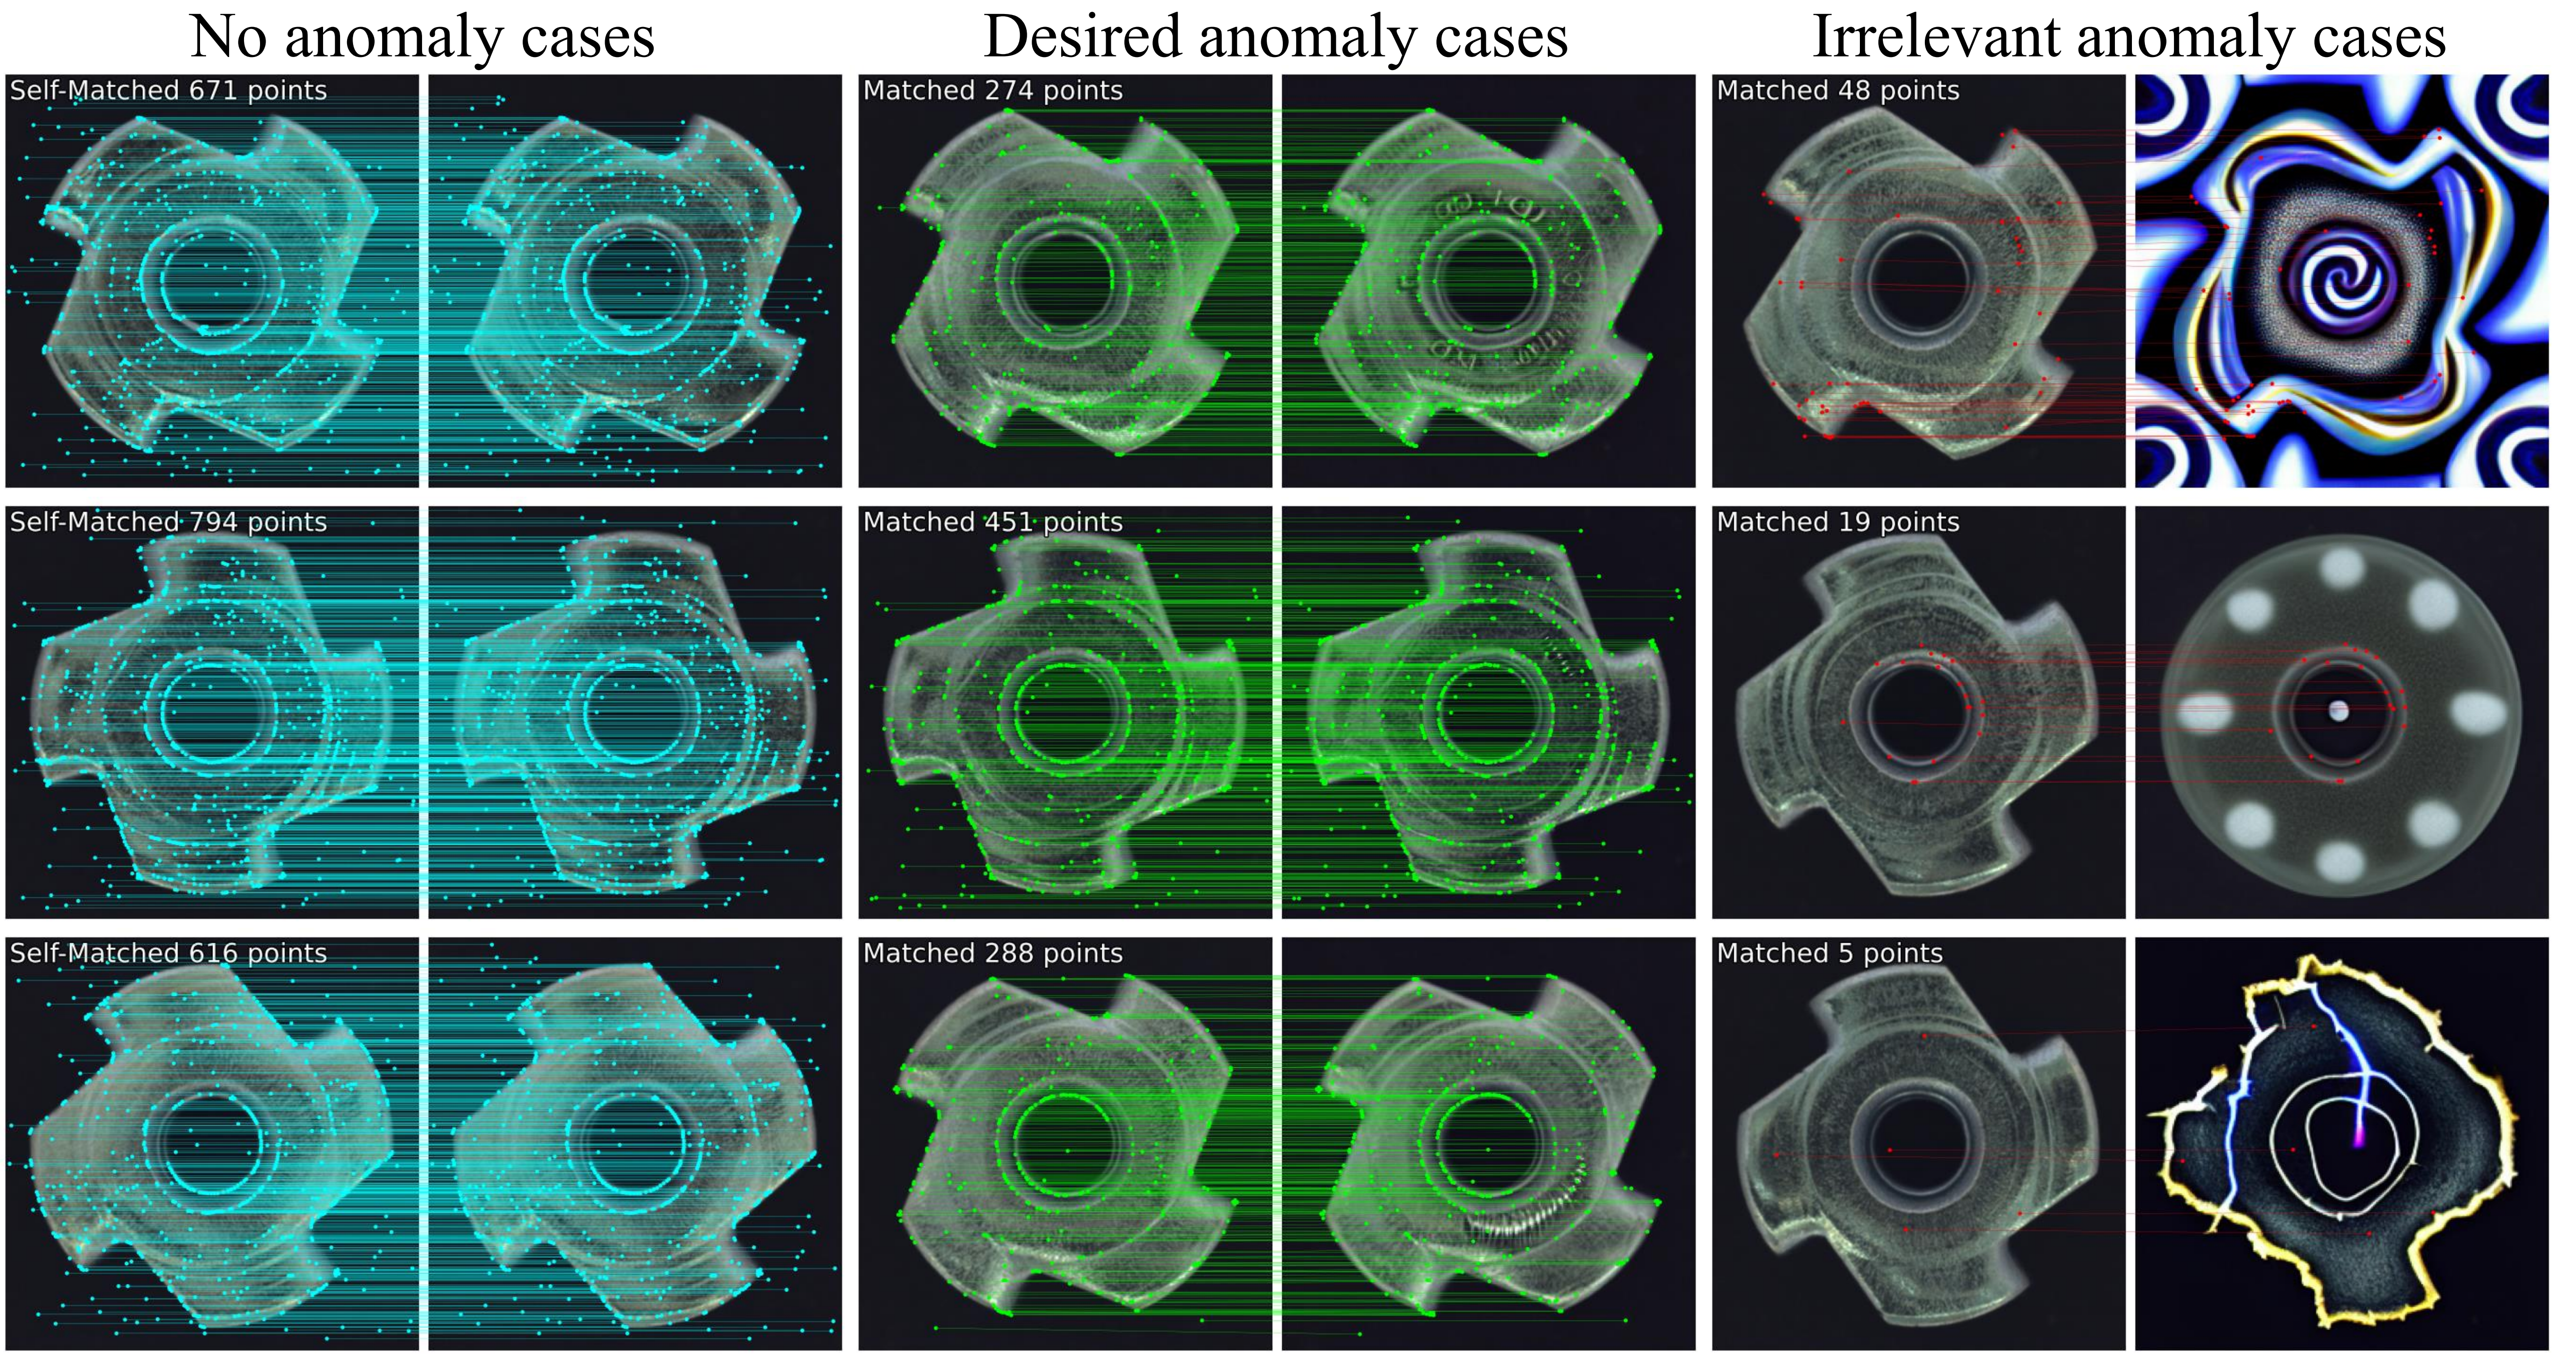
No anomaly cases
Desired anomaly cases
Irrelevant anomaly cases
Self-Matched 671 points
Matched 274 points
Matched 48 points
Self-Matched 794 points
Matched 451 points
Matched 19 points
Self-Matched 616 points
Matched 288 points
Matched 5 points

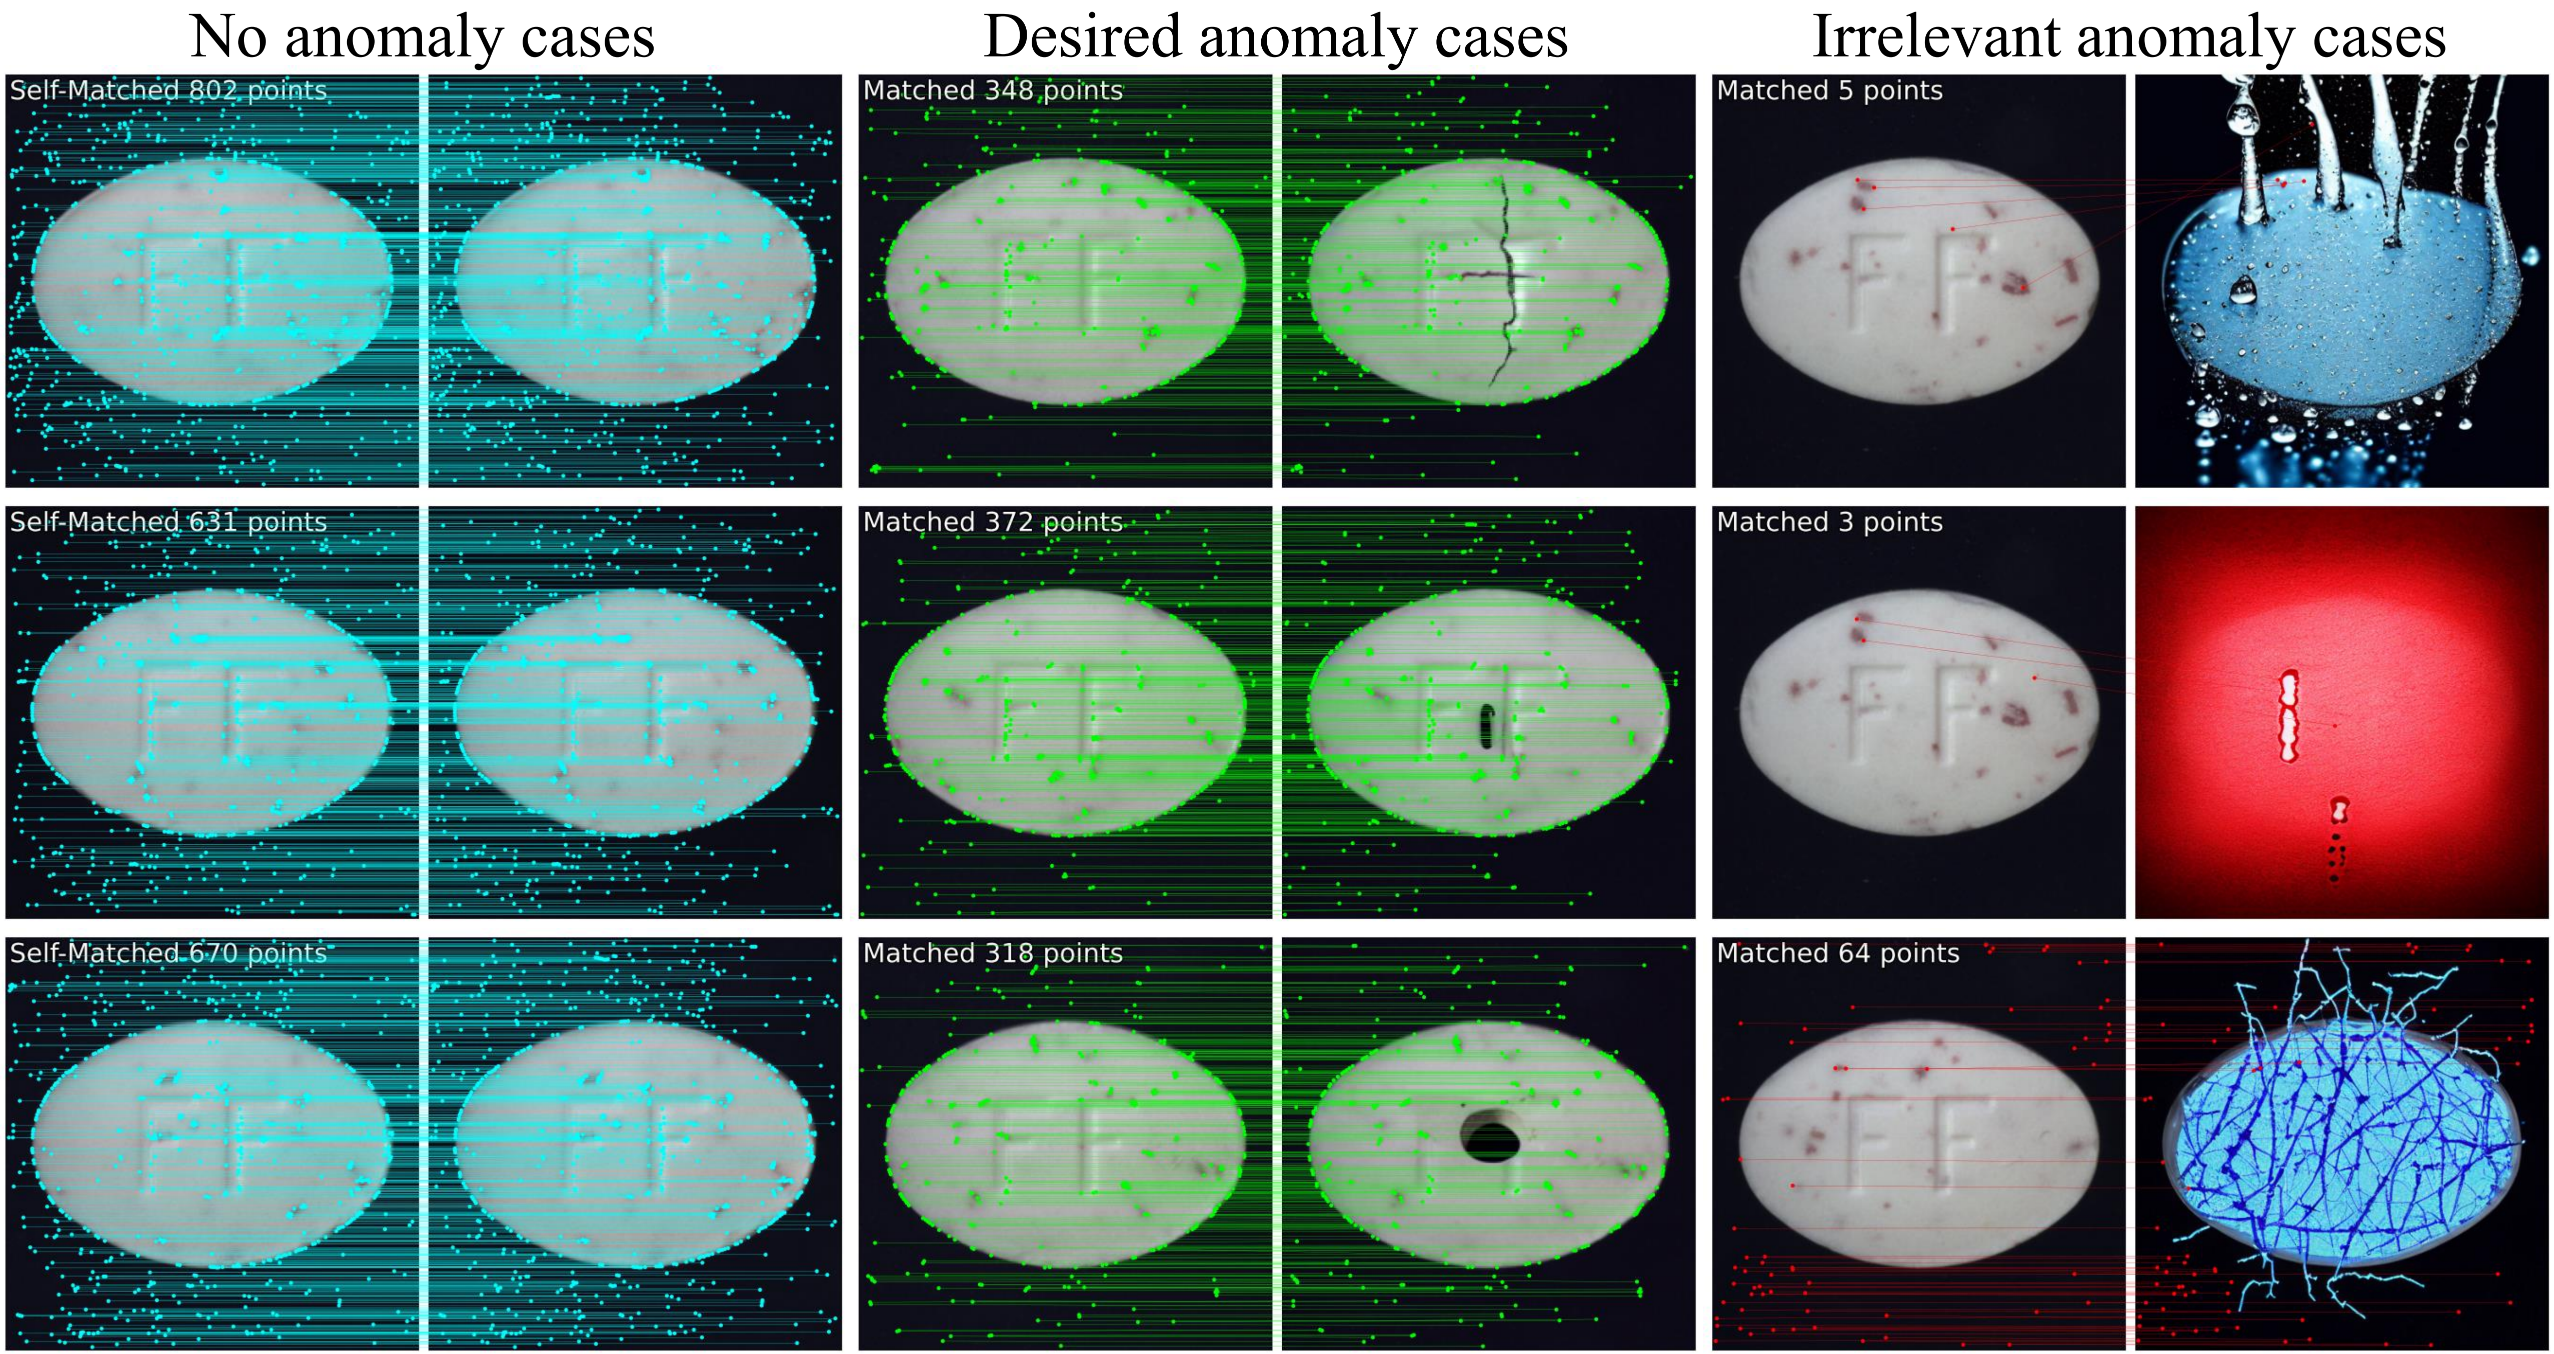
No anomaly cases
Desired anomaly cases
Irrelevant anomaly cases
Self-Matched 802 points
Matched 348 points
Matched 5 points
Self-Matched 631 points
Matched 372 points
Matched 3 points
Self-Matched 670 points
Matched 318 points
Matched 64 points

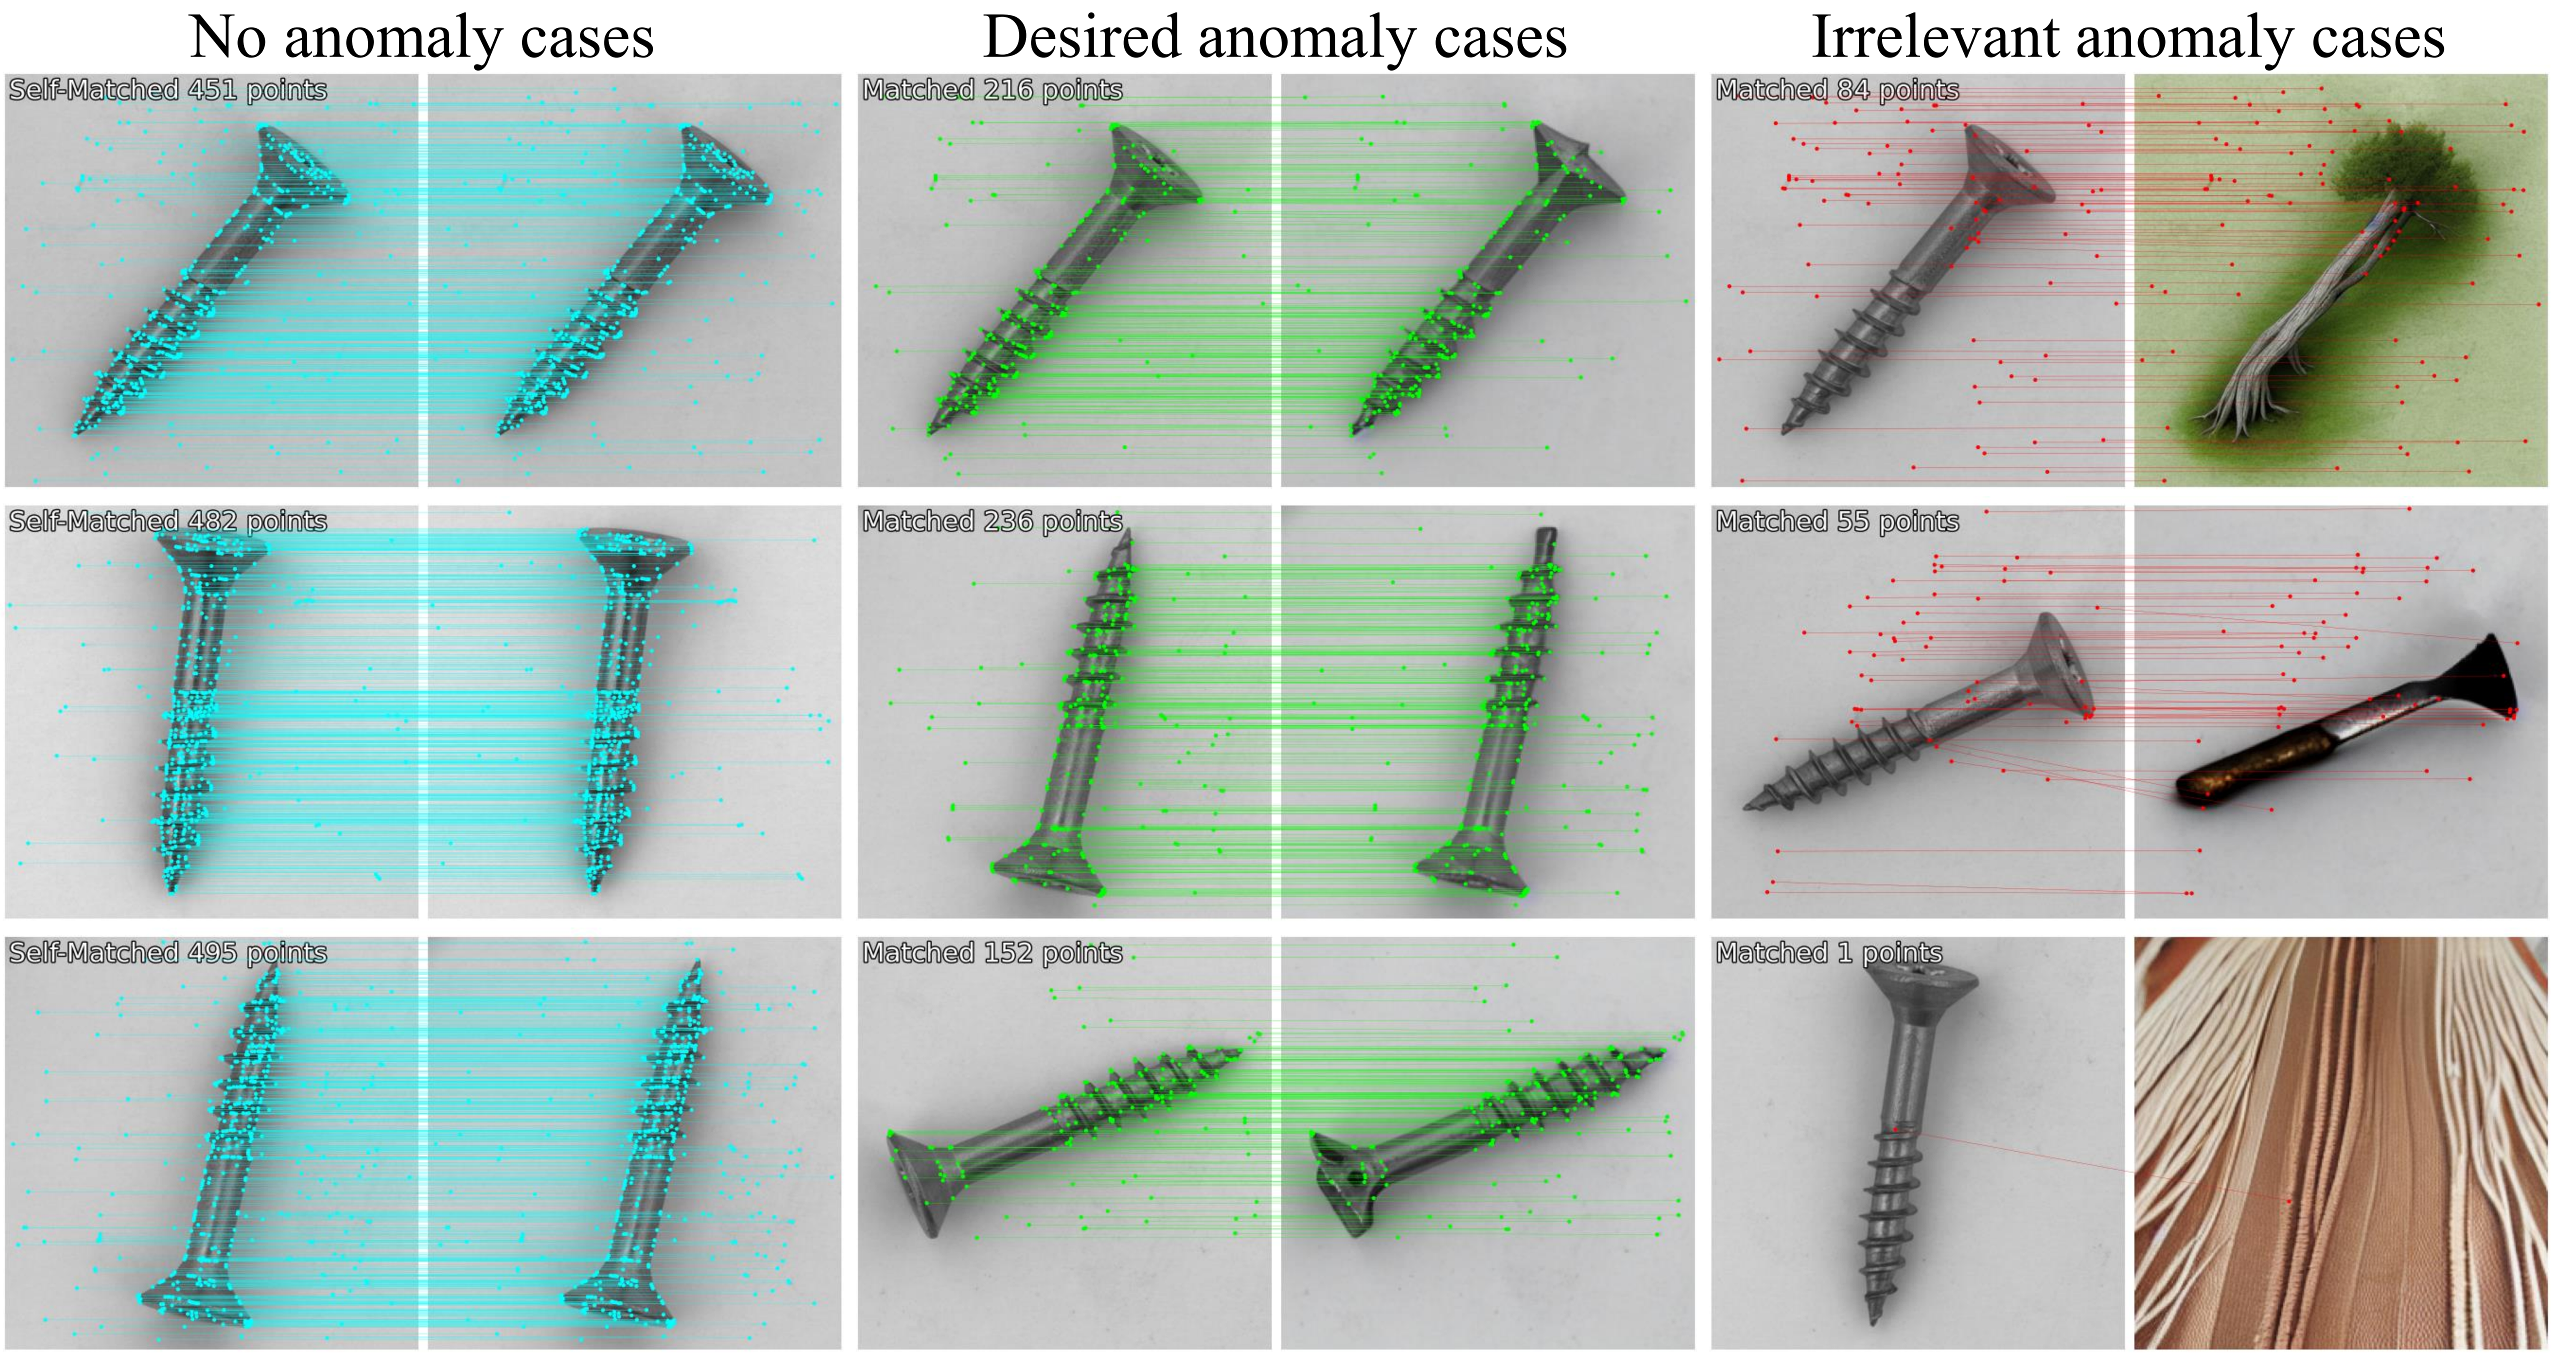
No anomaly cases
Desired anomaly cases
Irrelevant anomaly cases
Self-Matched 451 points
Matched 216 points
Matched 84 points
Self-Matched 482 points
Matched 236 points
Matched 55 points
Self-Matched 495 points
Matched 152 points
Matched 1 points

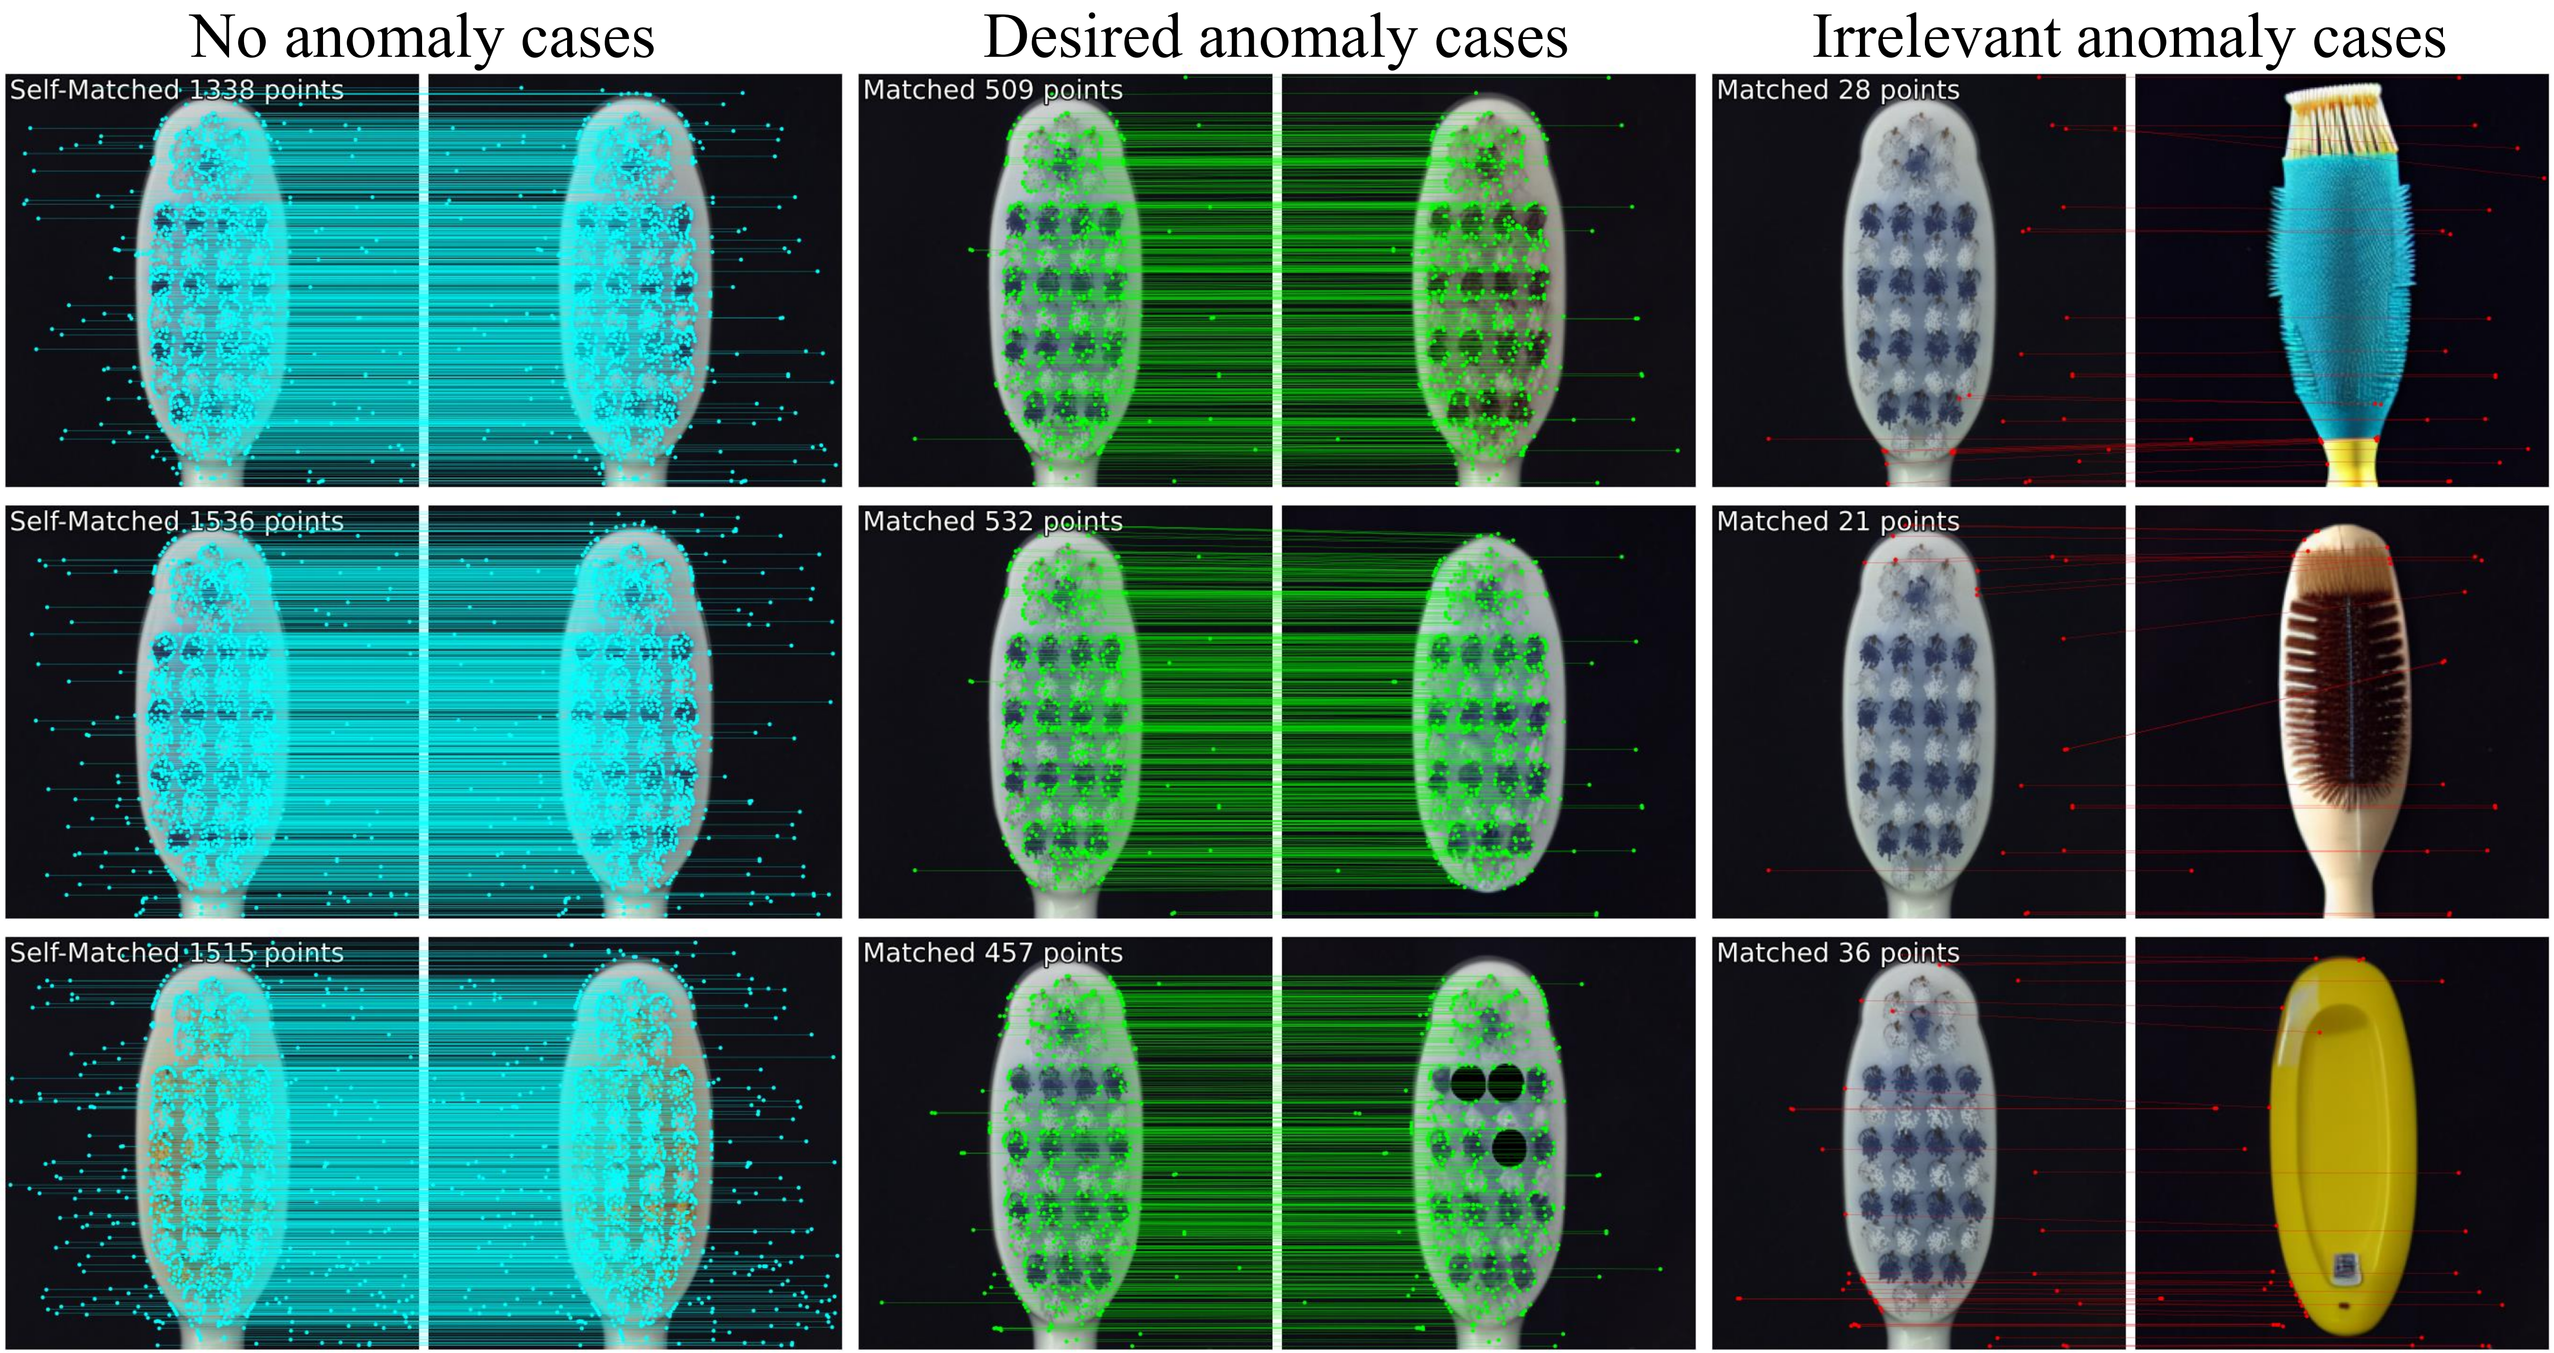
No anomaly cases
Desired anomaly cases
Irrelevant anomaly cases
Self-Matched 1338 points
Matched 509 points
Matched 28 points
Self-Matched 1536 points
Matched 532 points
Matched 21 points
Self-Matched 1515 points
Matched 457 points
Matched 36 points

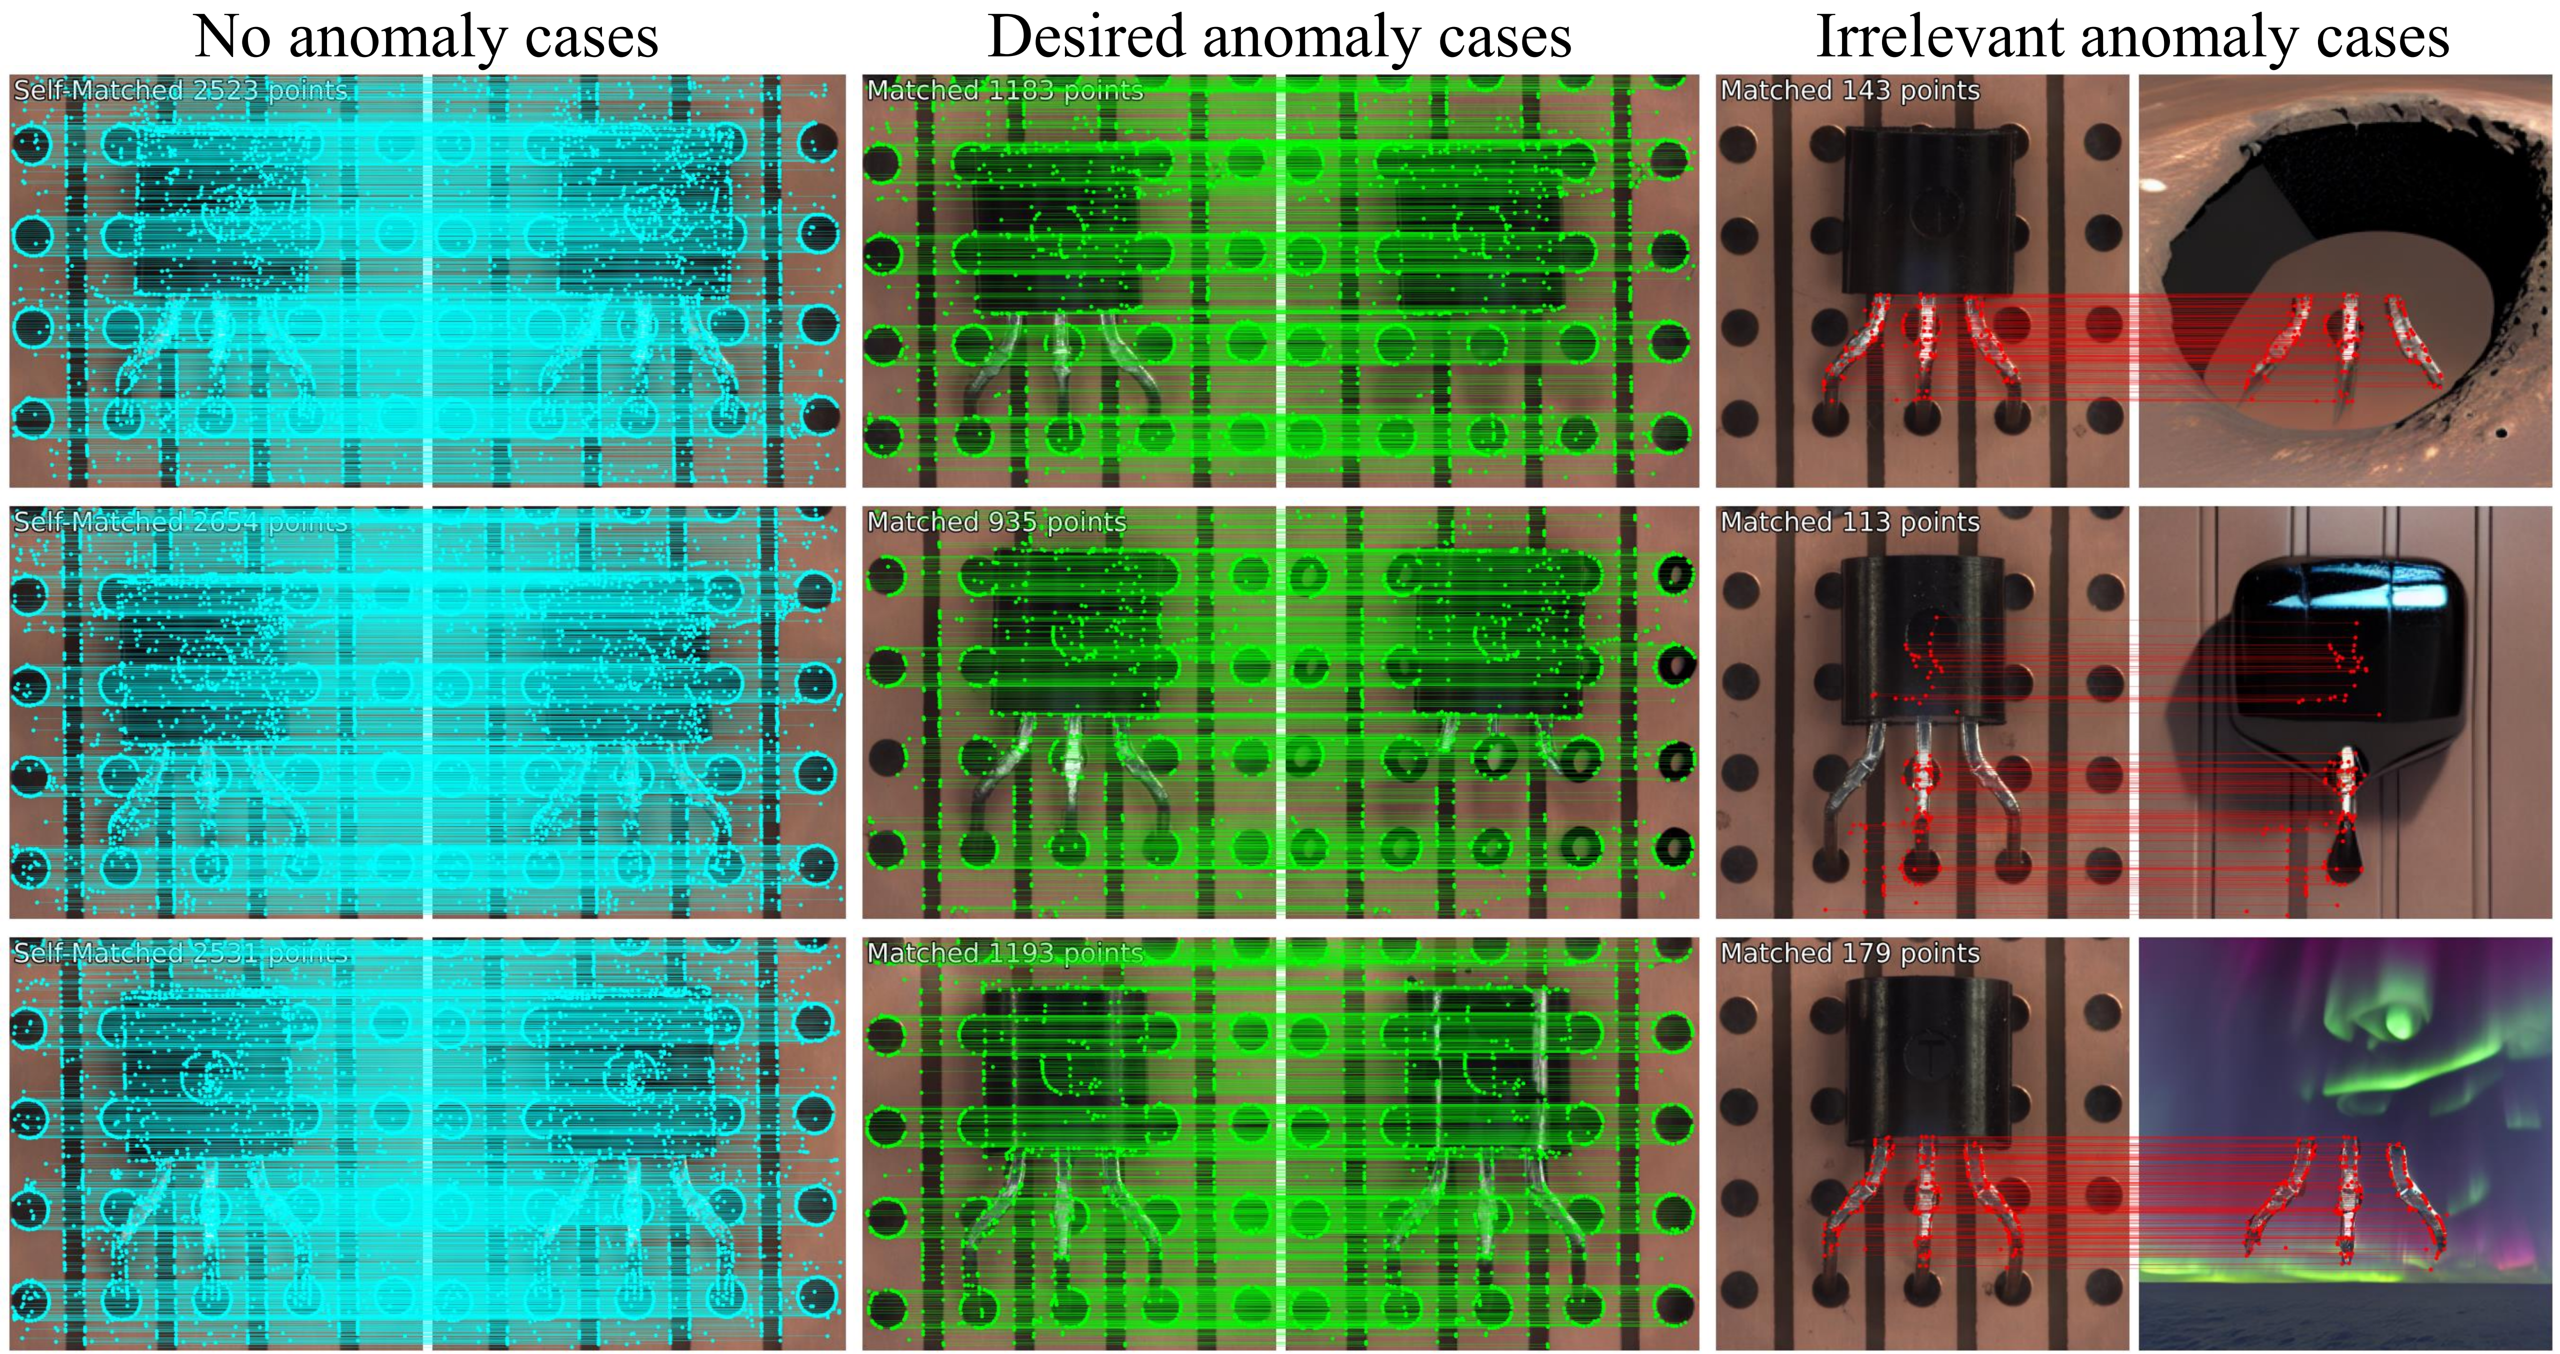

No anomaly cases
Desired anomaly cases
Irrelevant anomaly cases
Self-Matched 2523 points
Matched 1183 points
Matched 143 points
Self-Matched 2654 points
Matched 935 points
Matched 113 points
Self-Matched 2531 points
Matched 1193 points
Matched 179 points

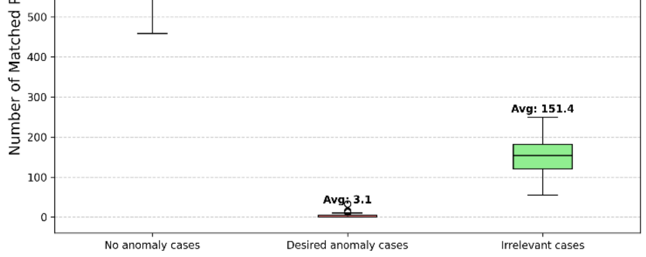


Bottle

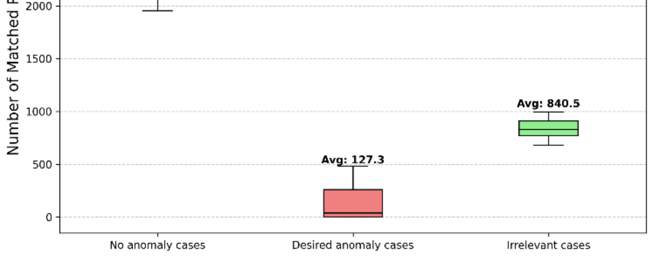


Cable

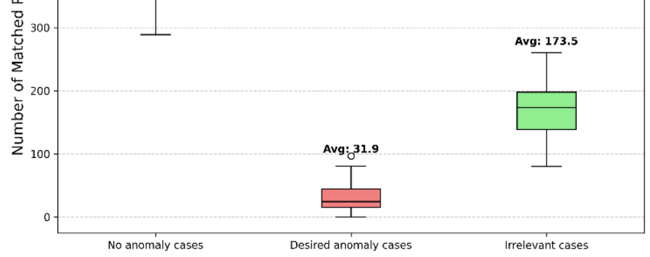


Capsule

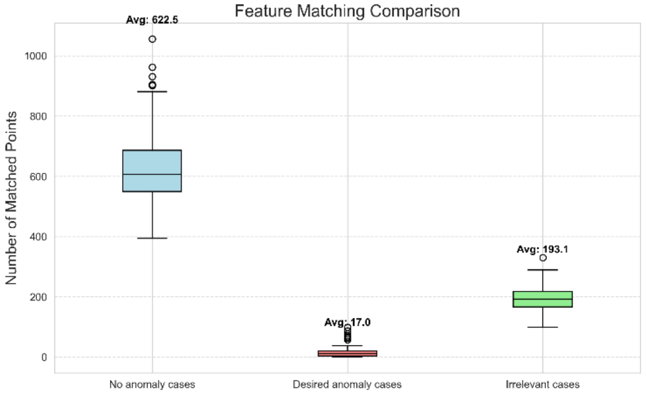


Hazelnut

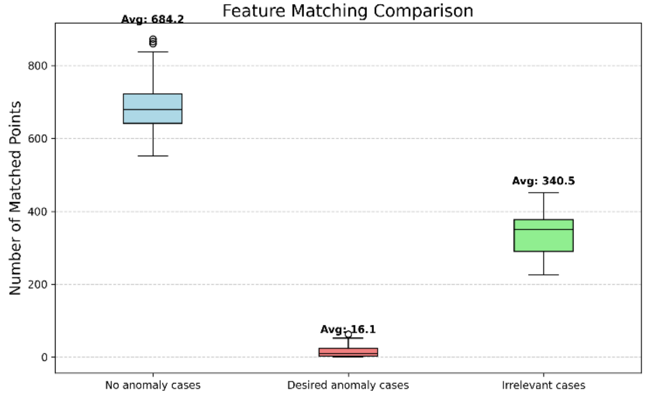


Metal nut

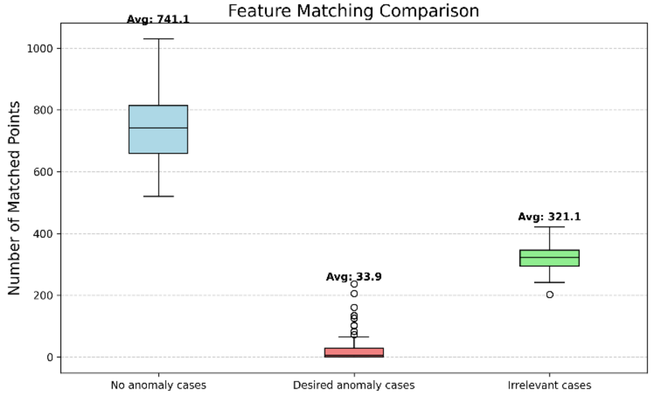


Pill

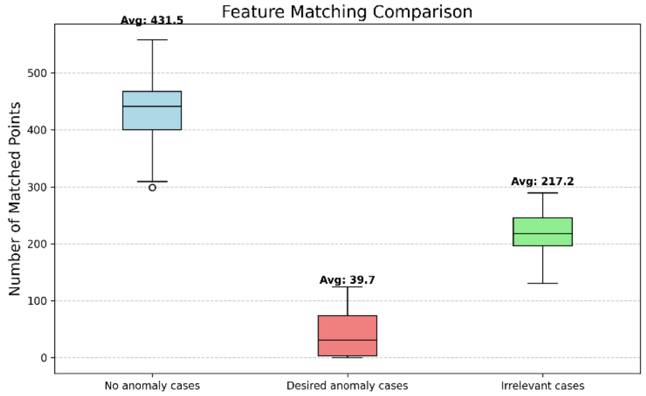


Screw

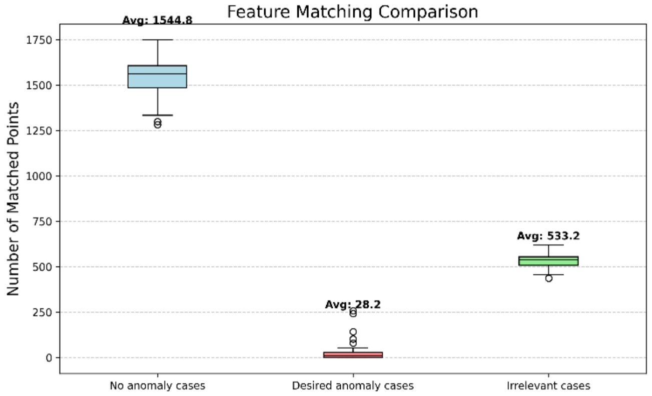


Toothbrush

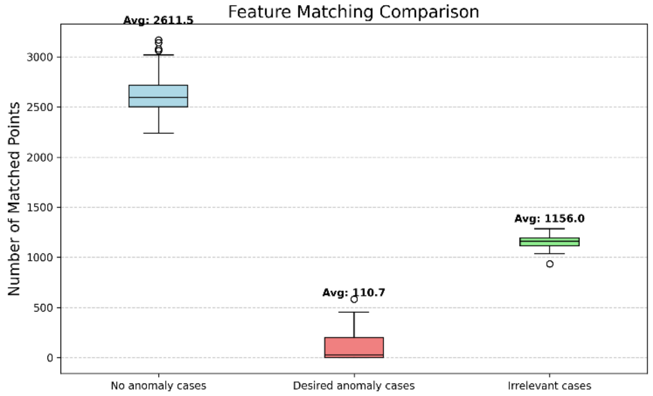


Transistor
